# Supplementary material for: Enhancing Empathic Accuracy: Penalized Functional Alignment Method to Correct Temporal Misalignment in Real-time Emotional Perception
Source: arXiv:2409.05343 source file (2025-08-07)

# Estimated correlations between perceivers and targets

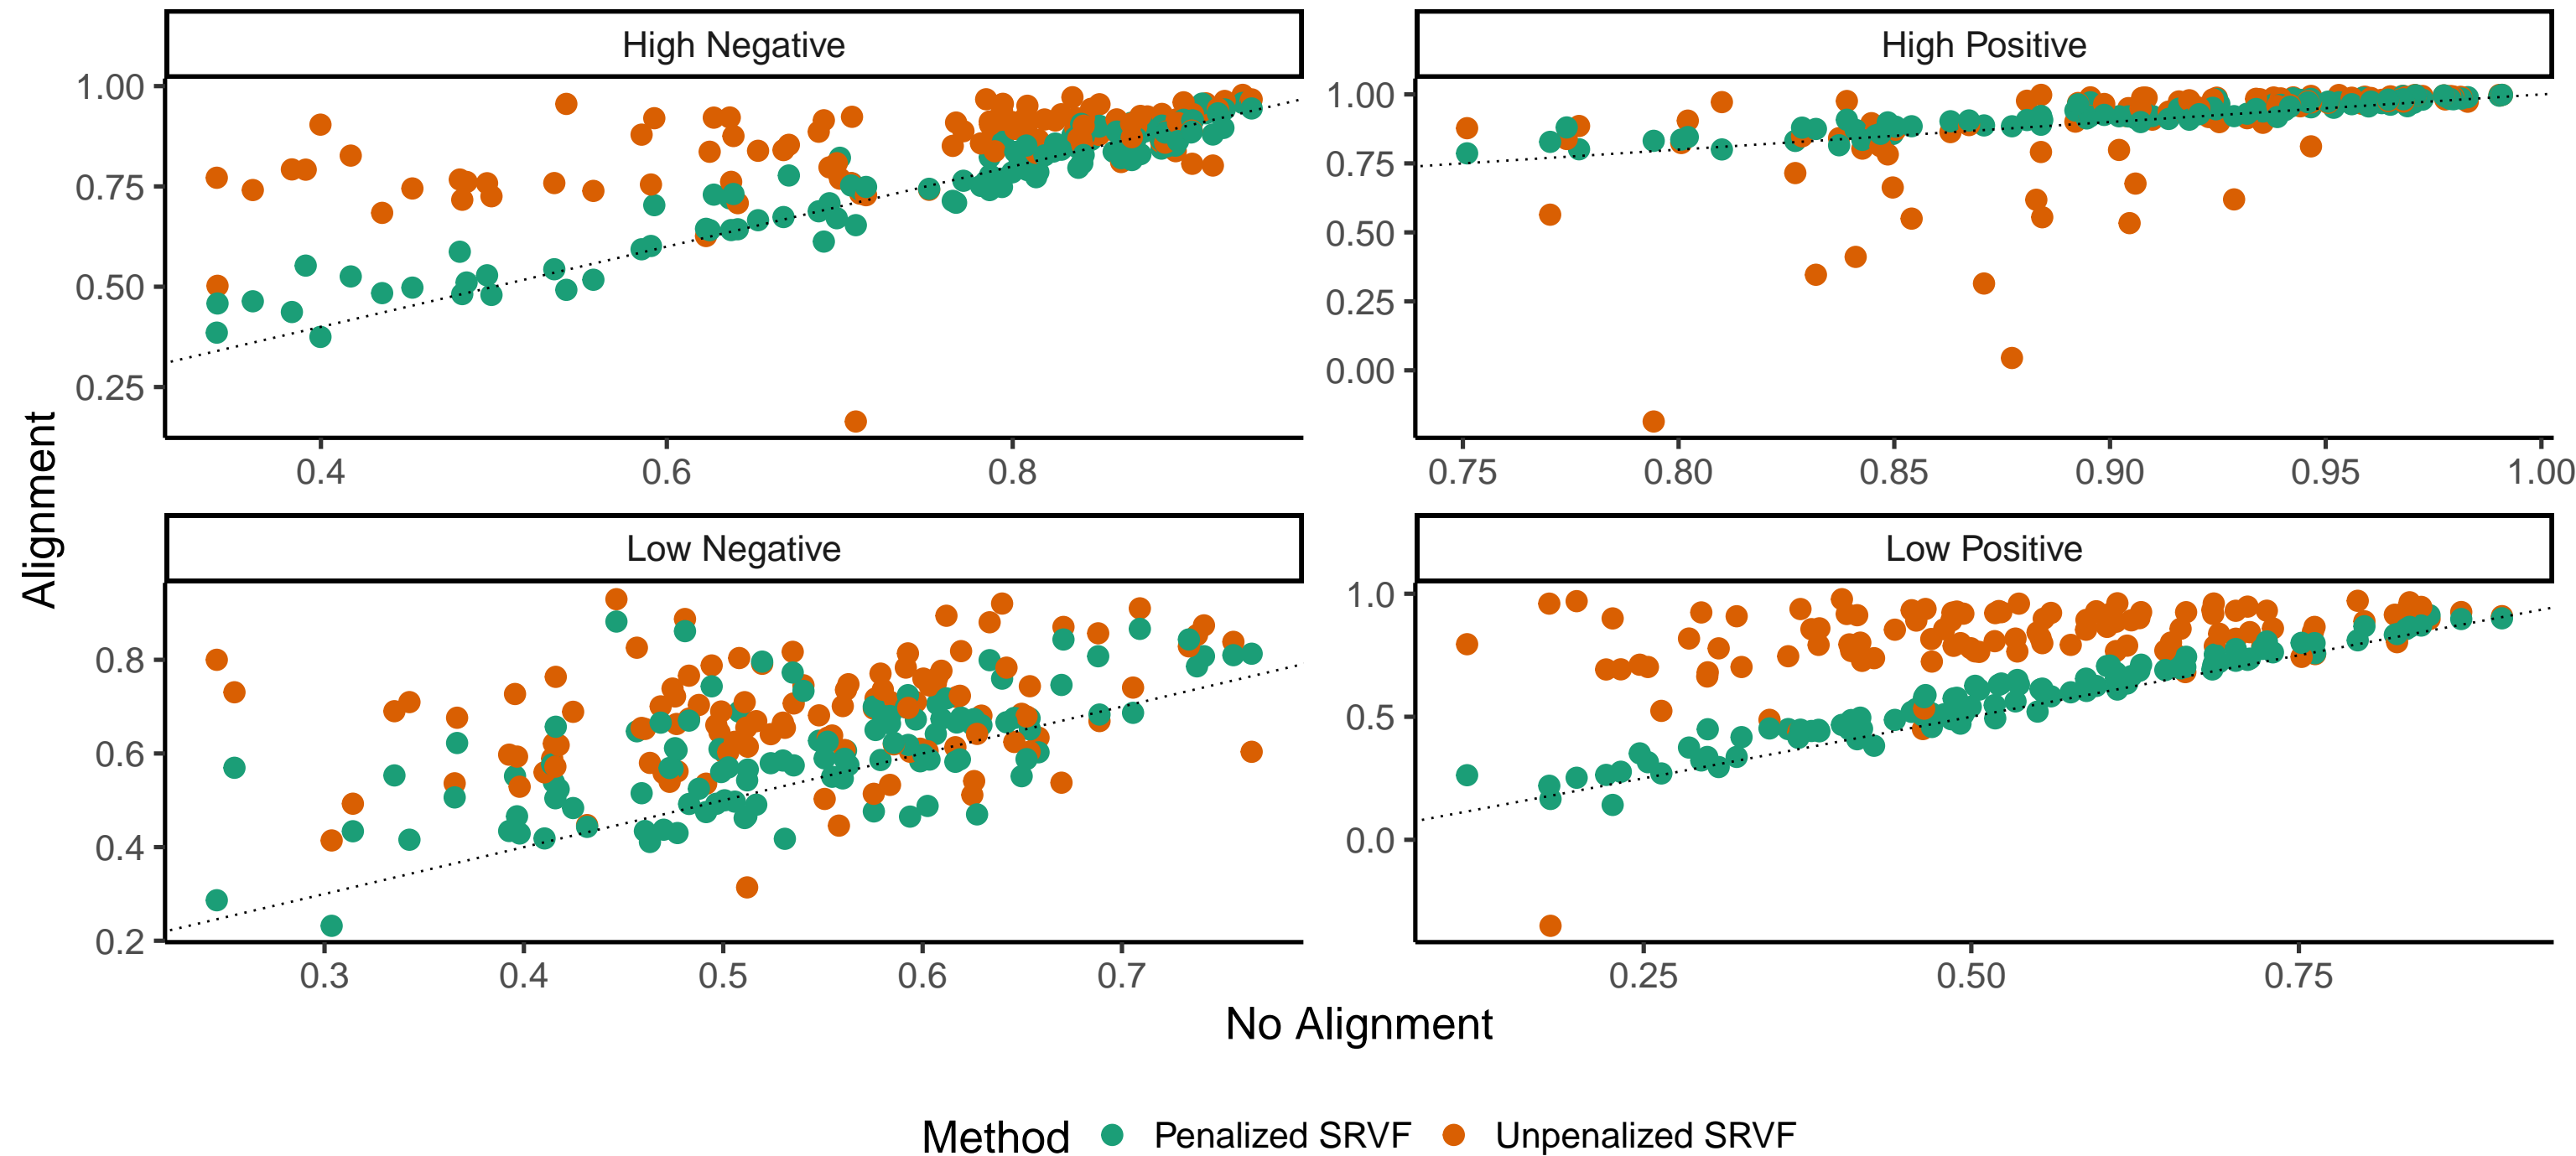

# L2 distance

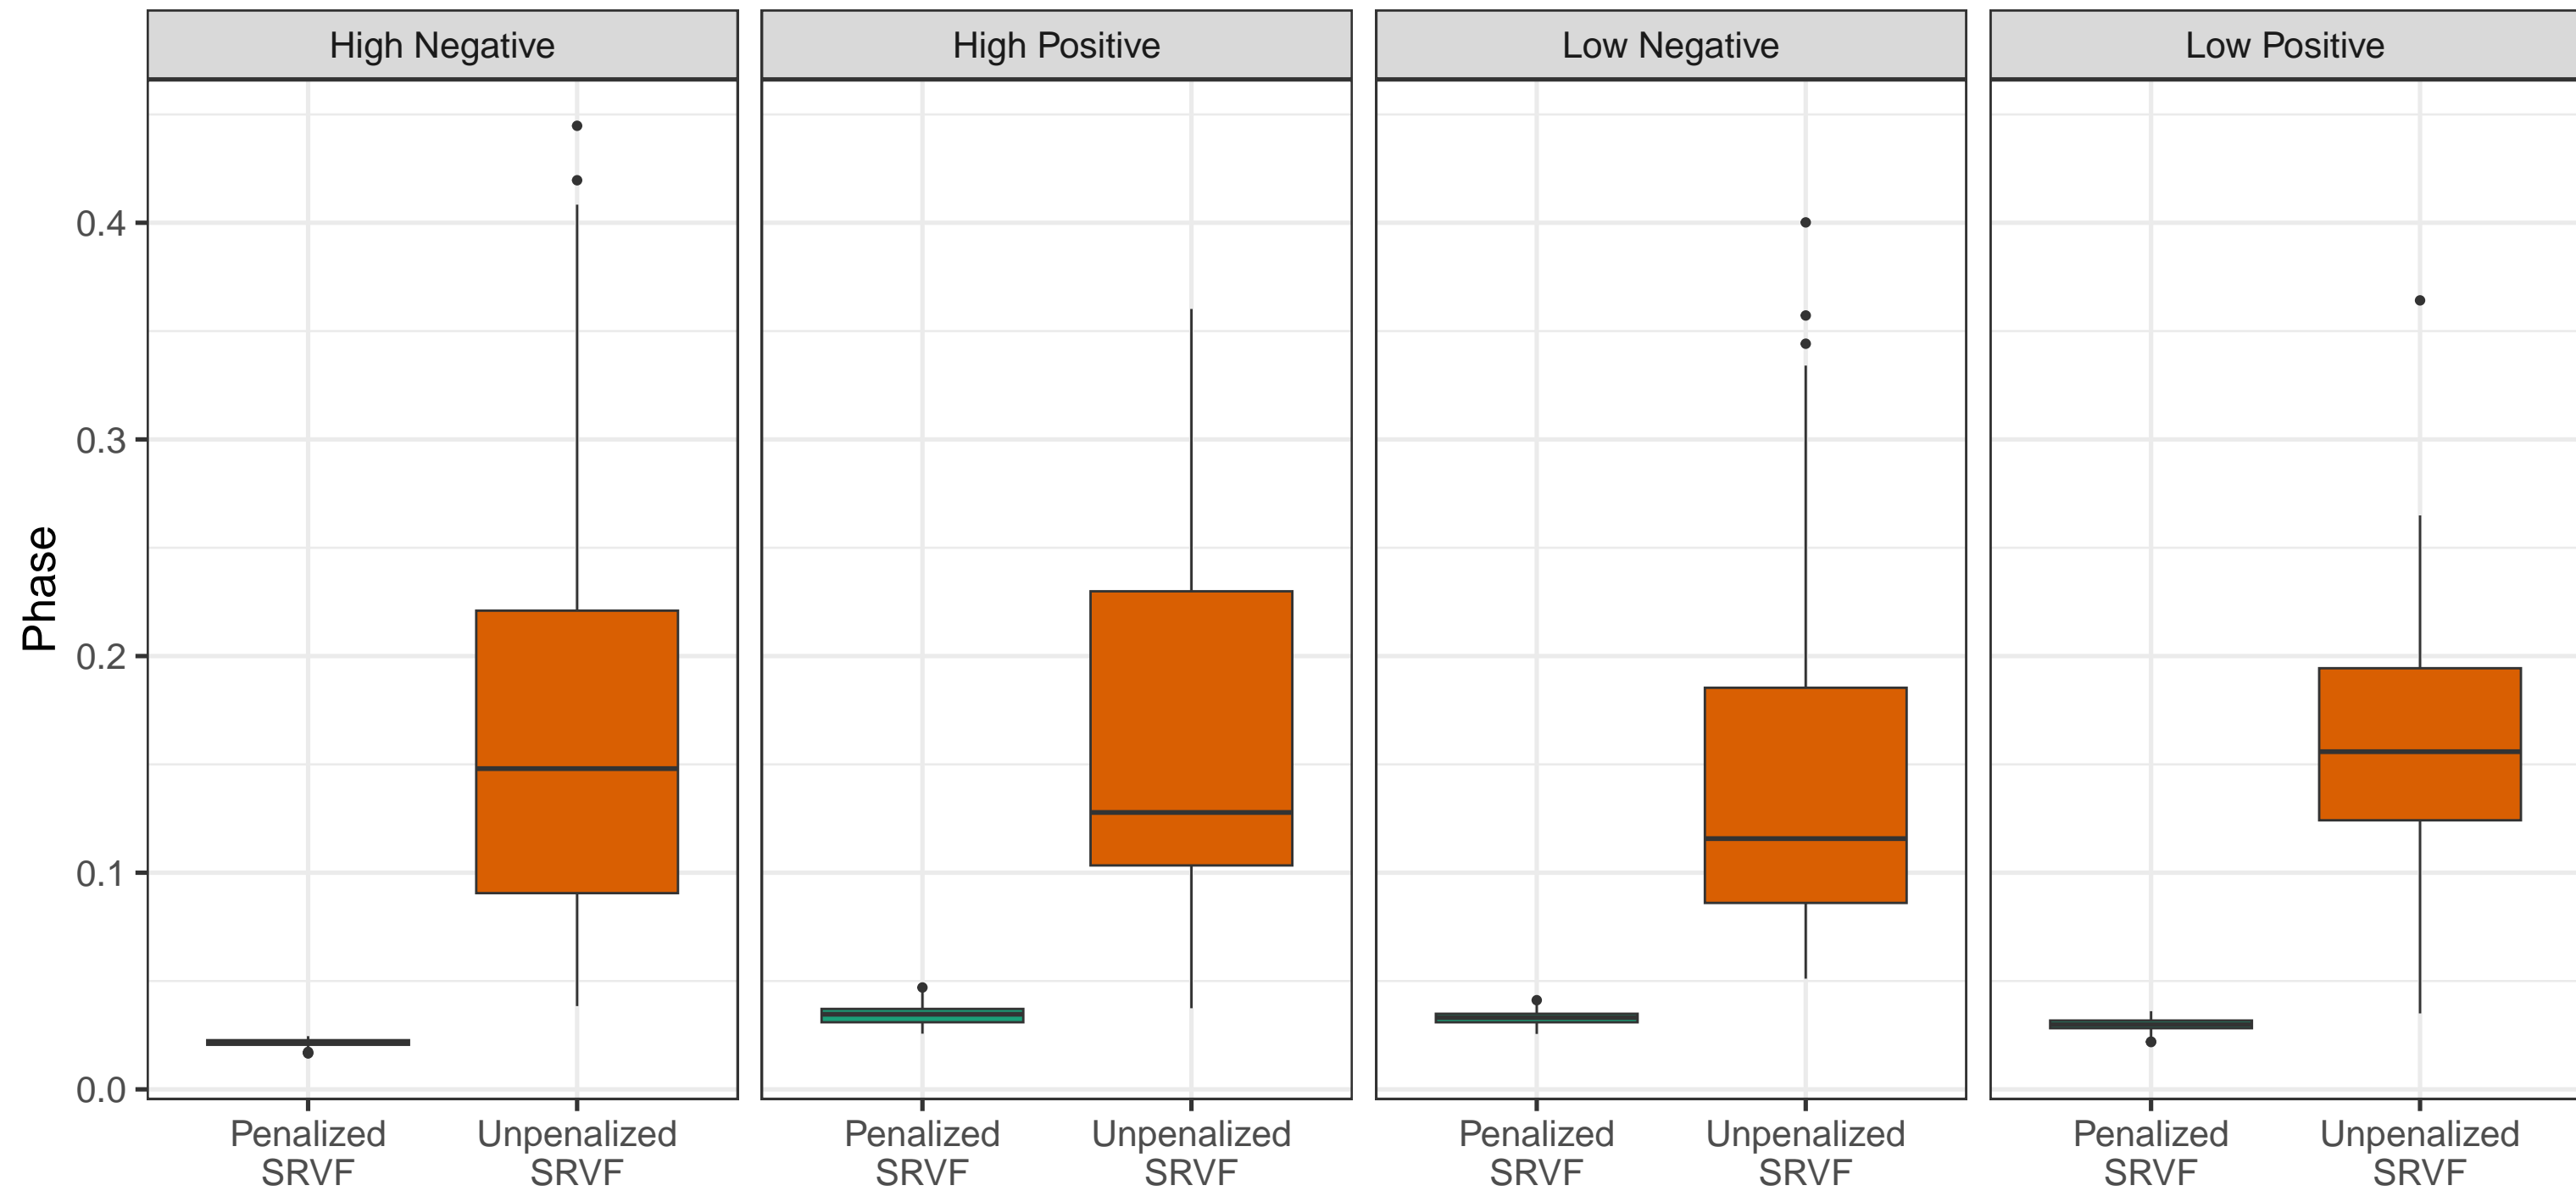

Fisher-Rao metric

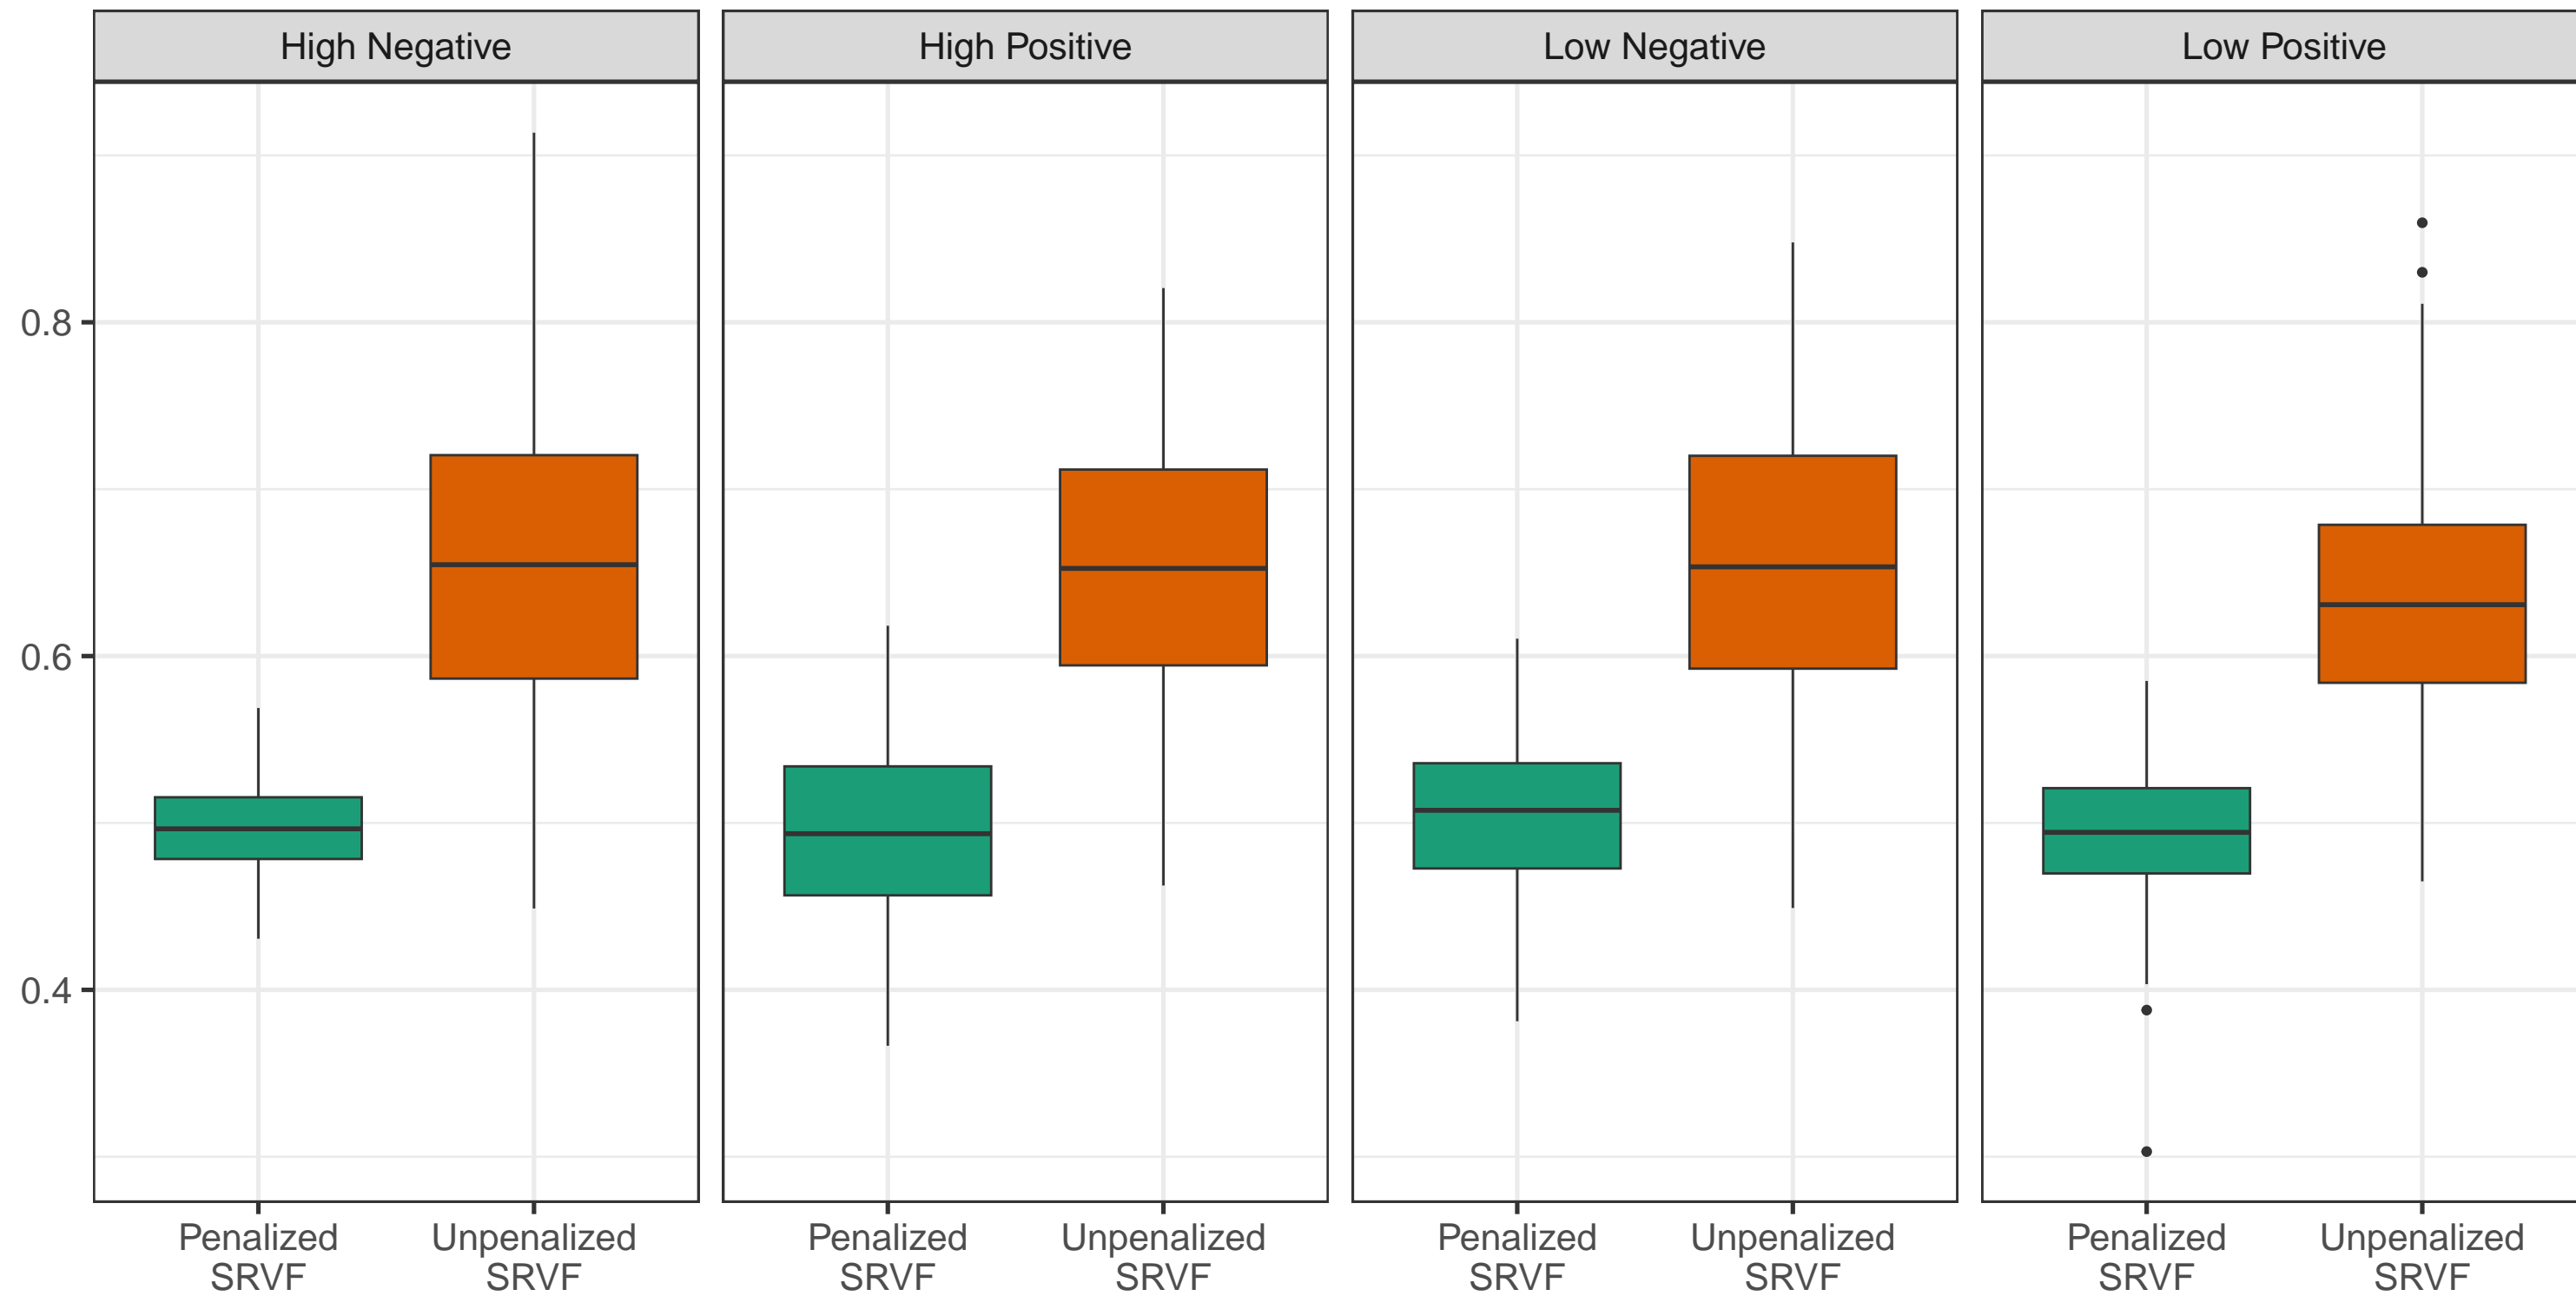

# Estimated correlations between perceivers and targets

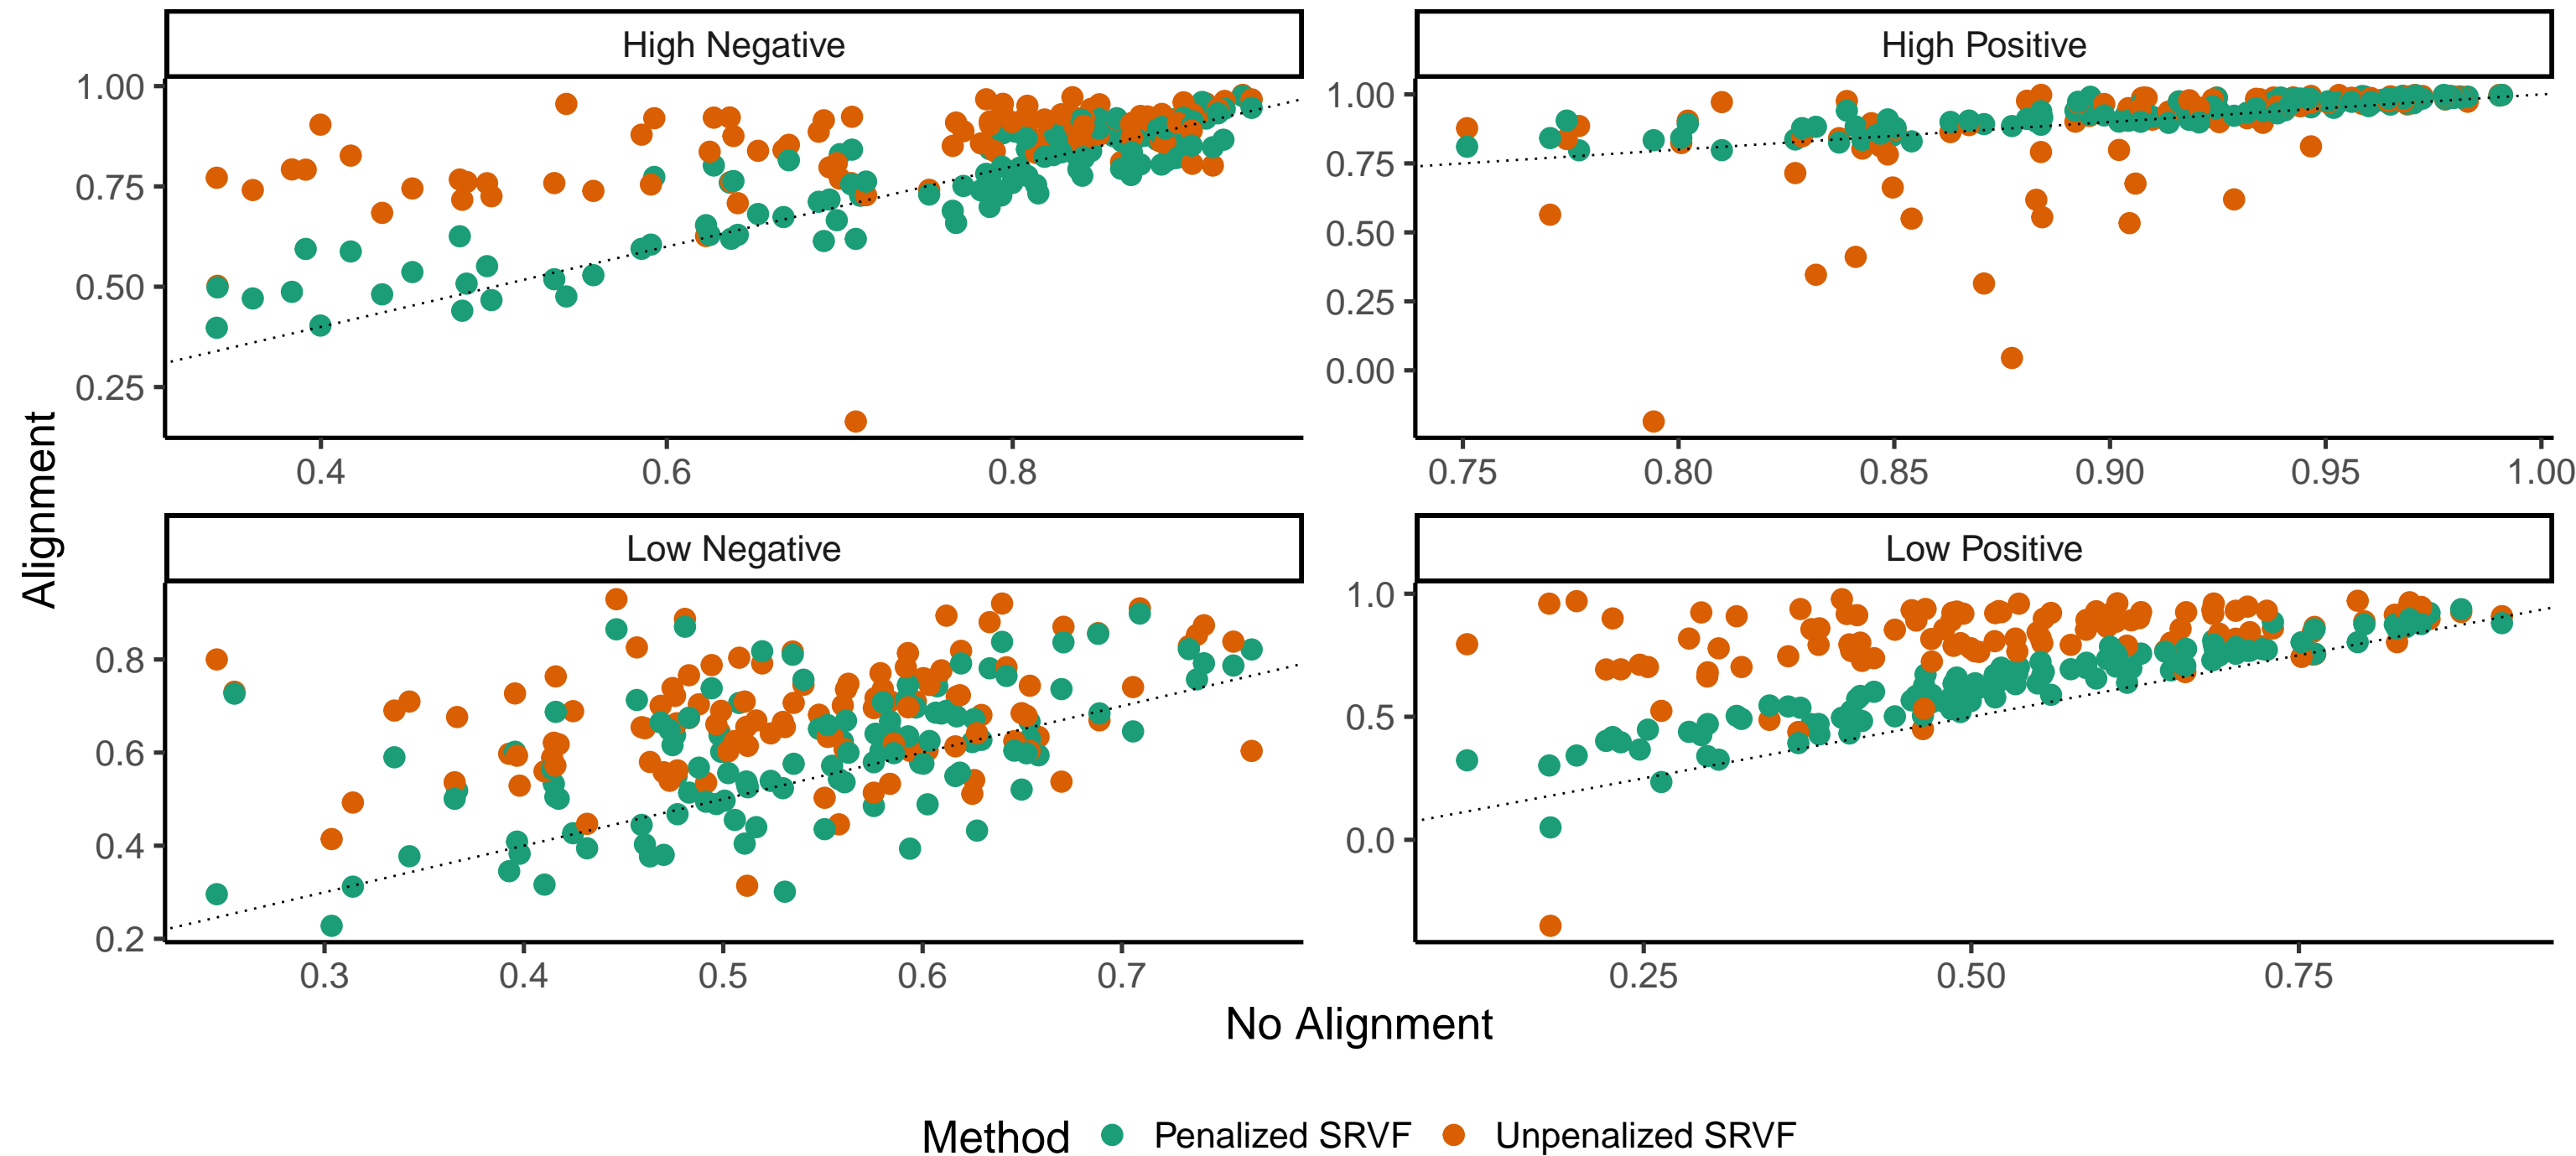

# L2 distance

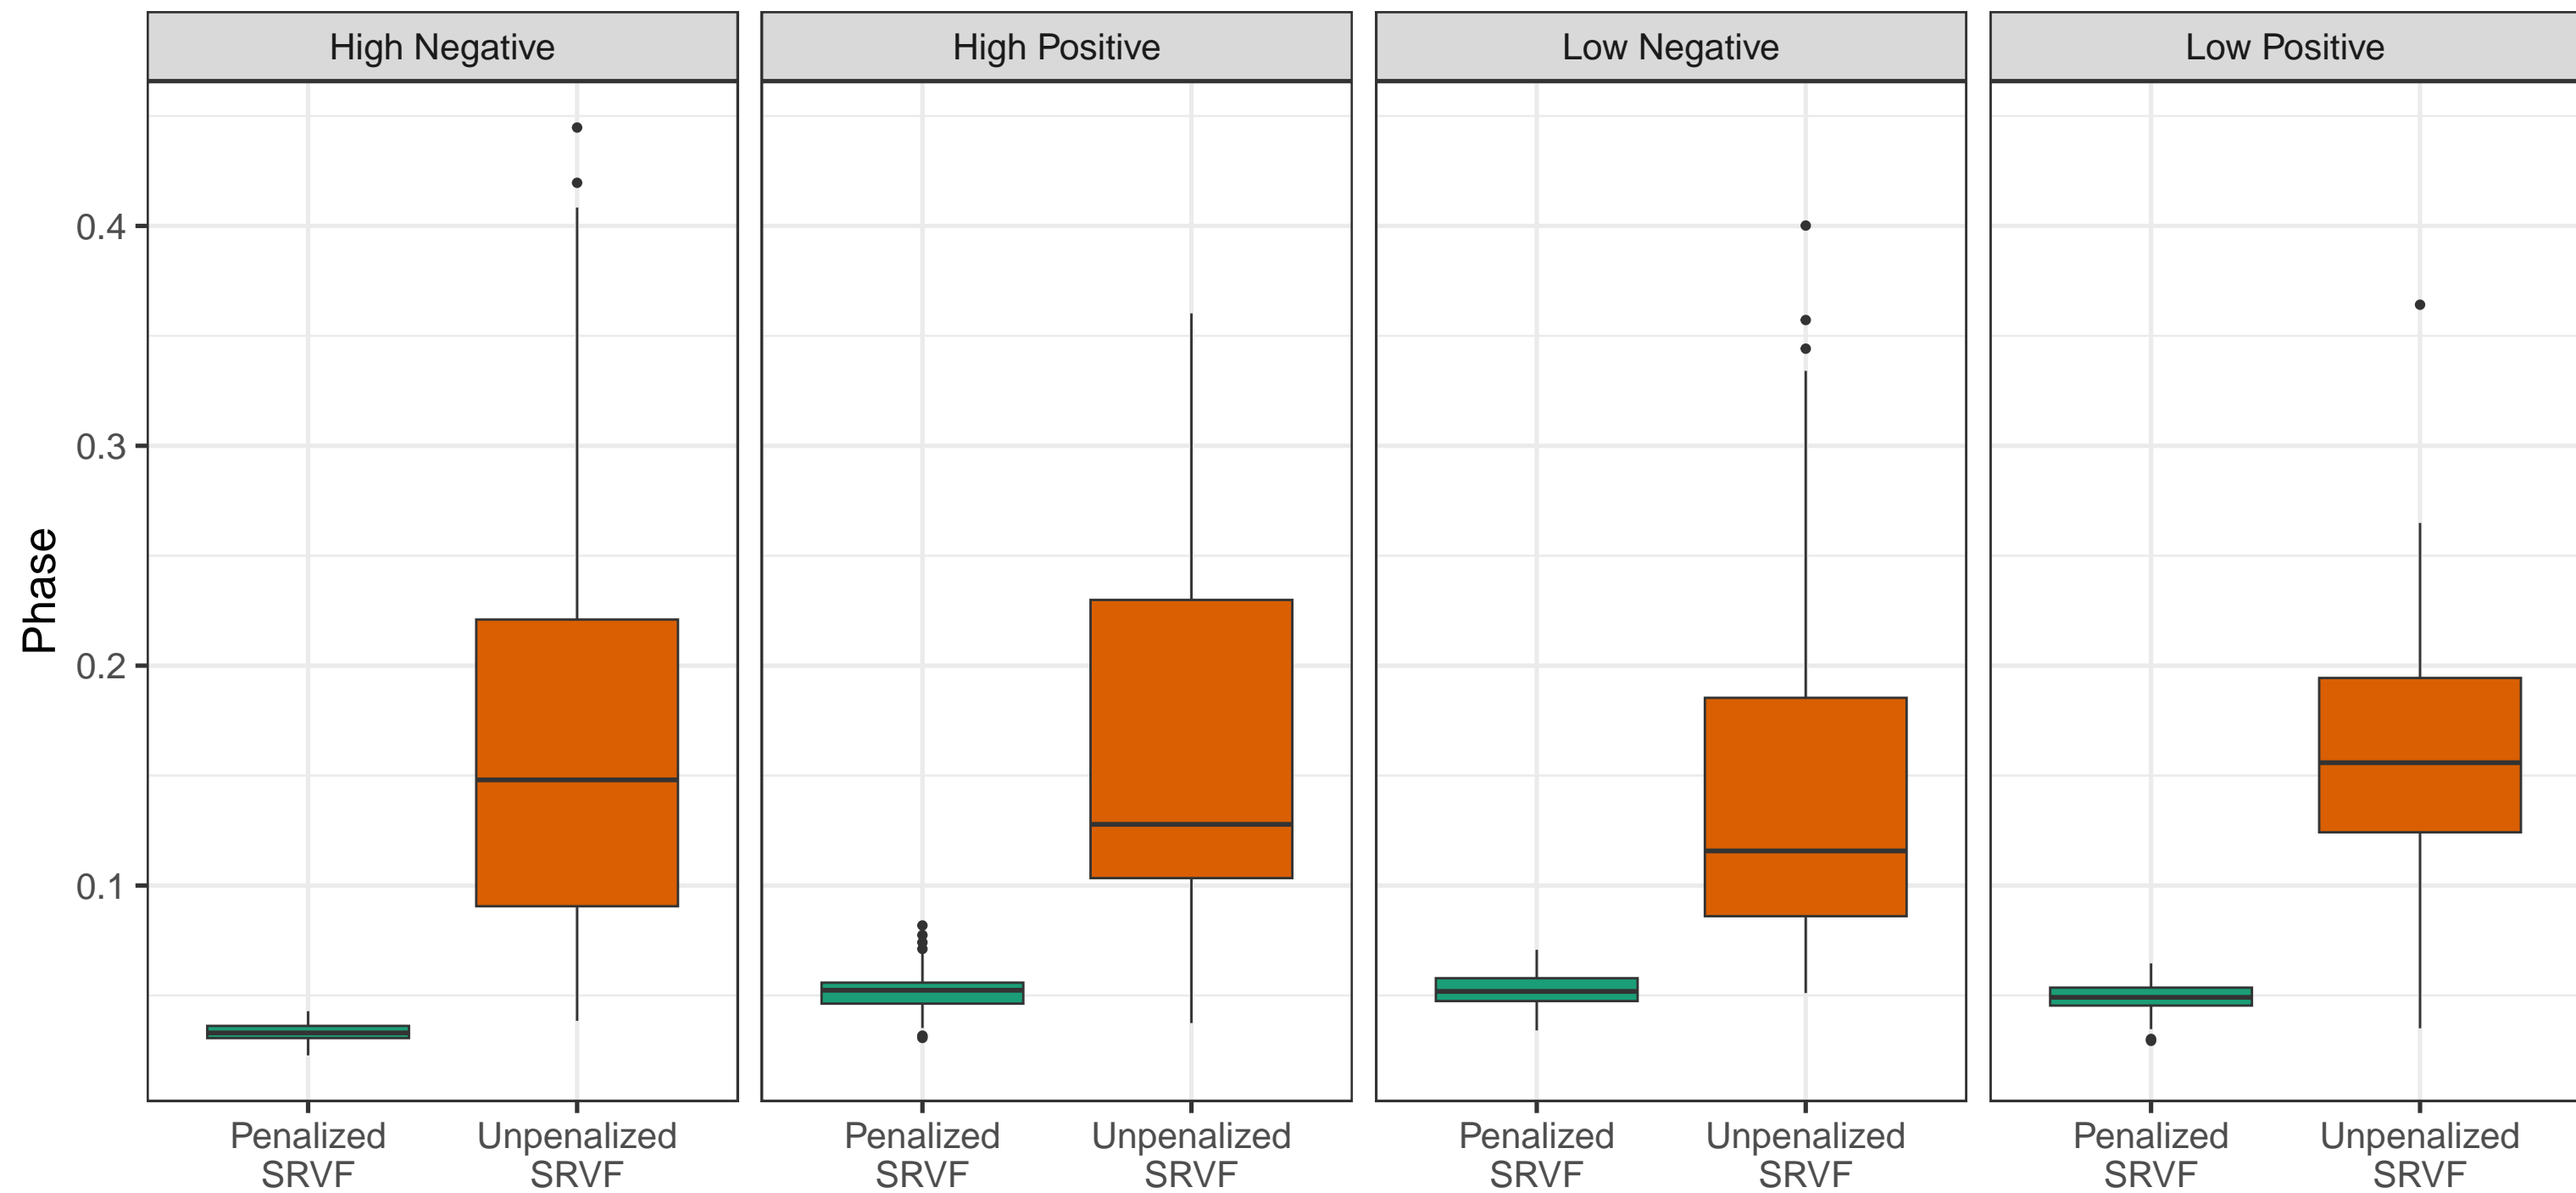

Fisher-Rao metric

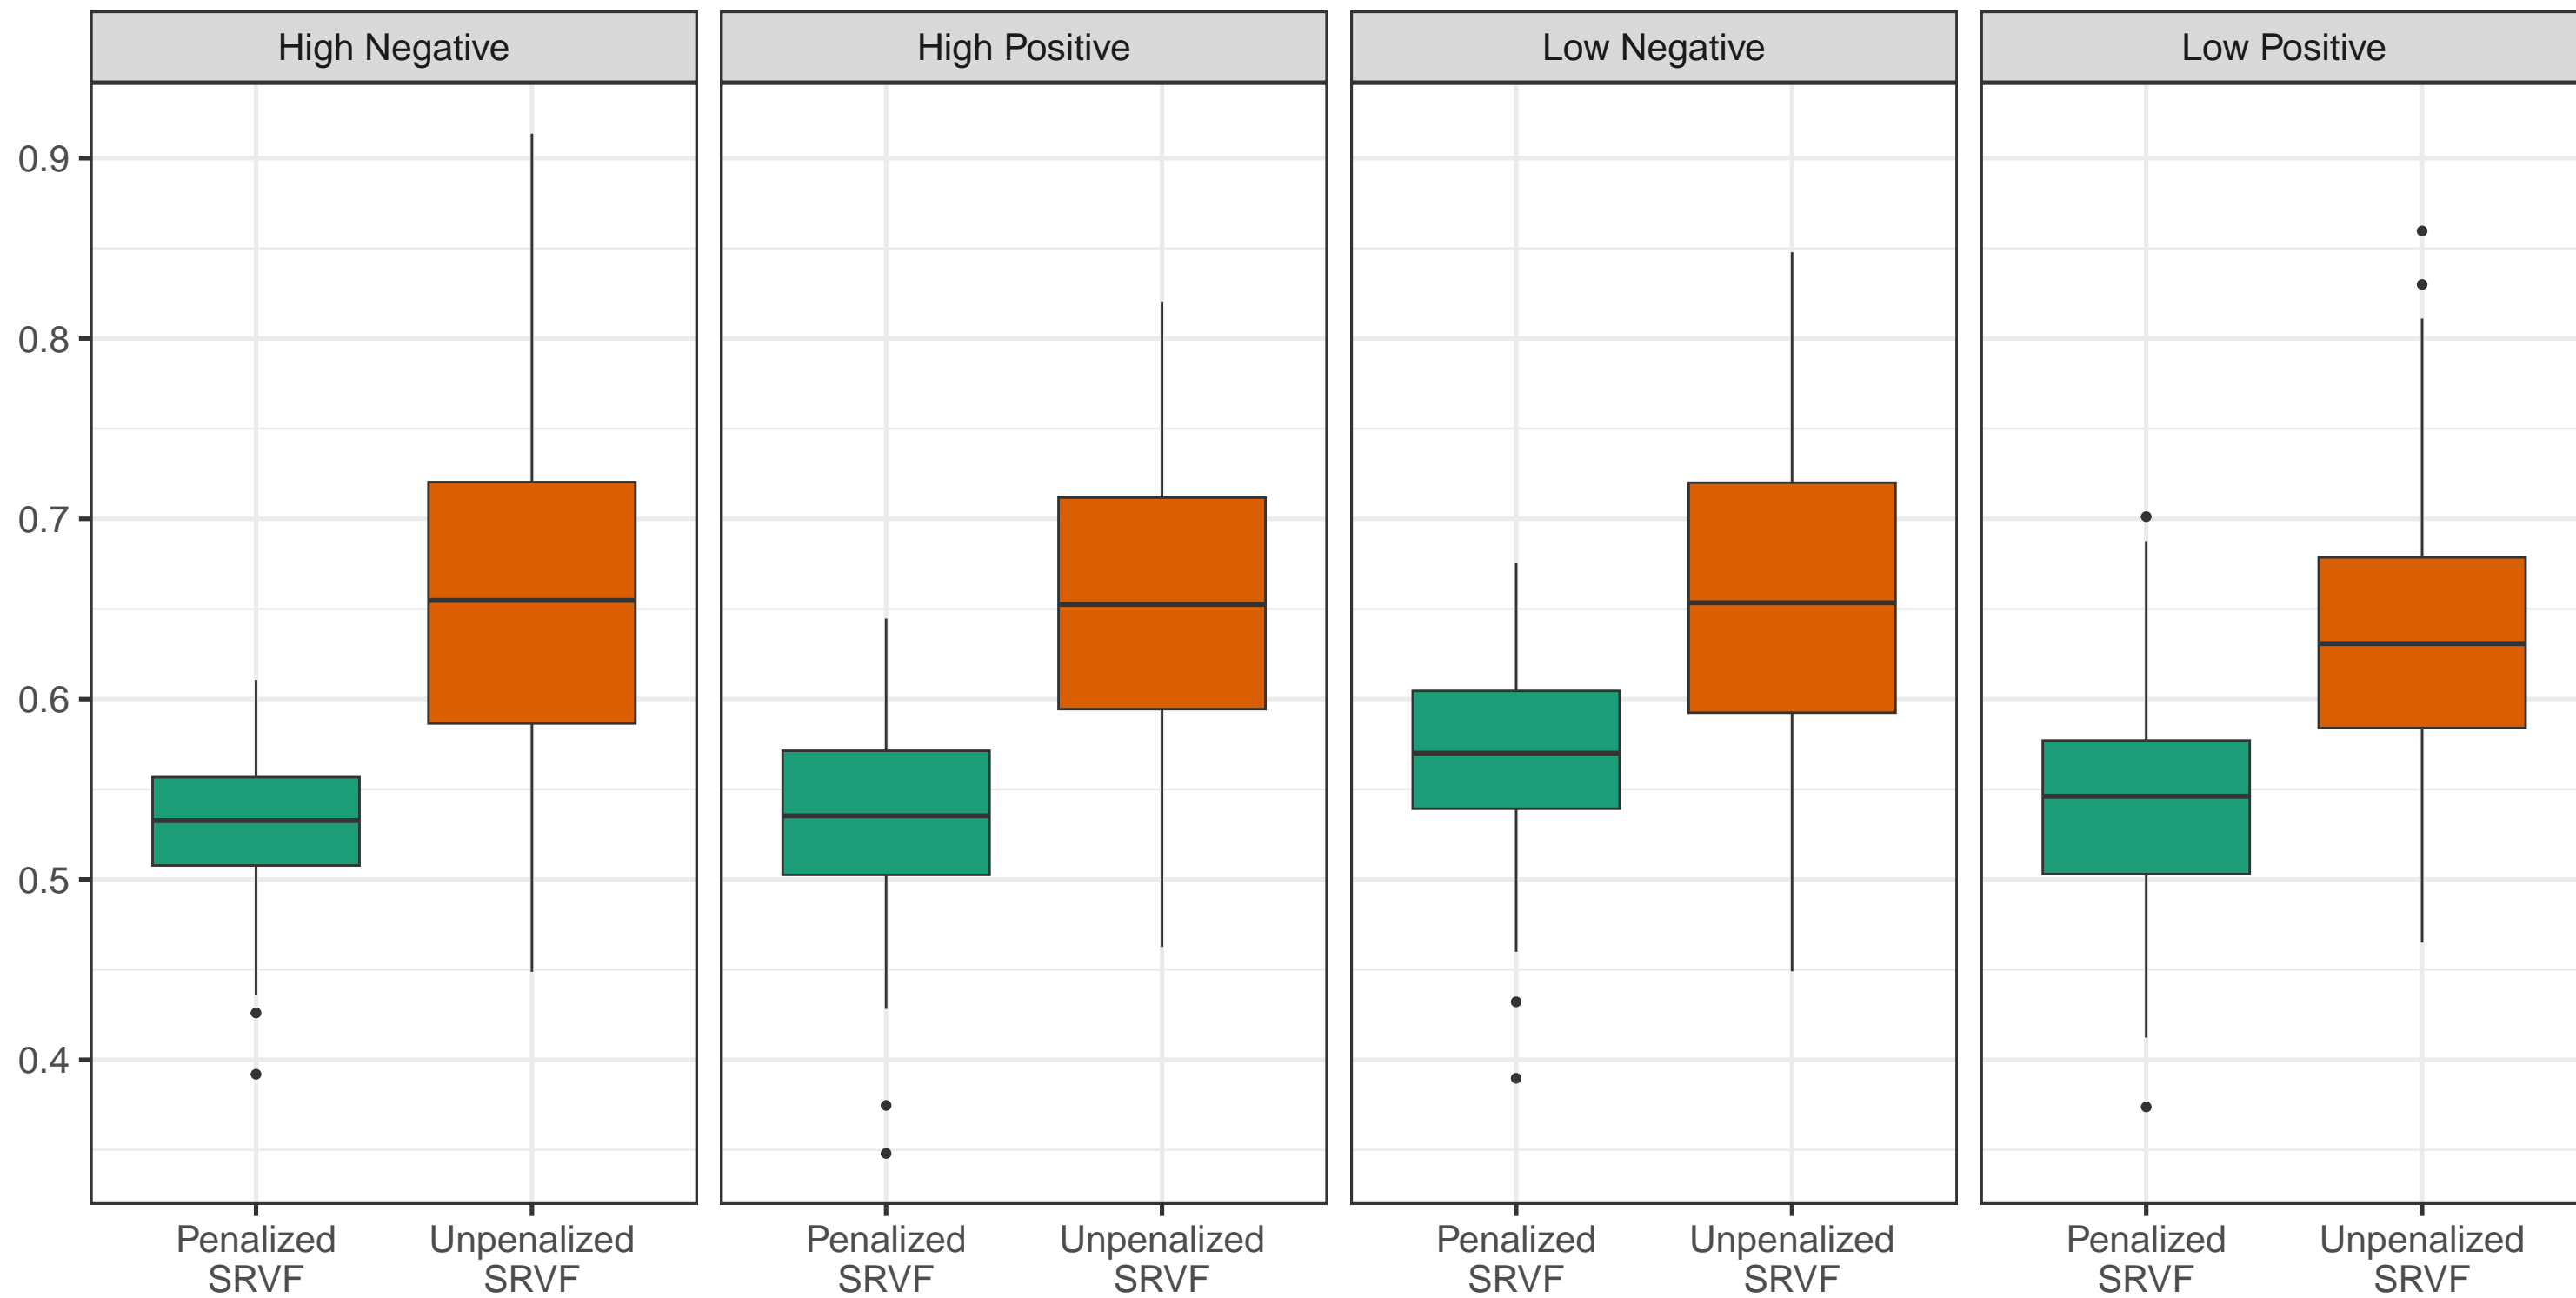

Supplement: Supplementary file 1 [file Delvin_new_plots_rmoutliers_18022024_appendix.pdf]
