# Supplementary material for: Enhancing Empathic Accuracy: Penalized Functional Alignment Method to Correct Temporal Misalignment in Real-time Emotional Perception
Source: arXiv:2409.05343 source file (2025-08-07)

# Correlations on f

Alignment

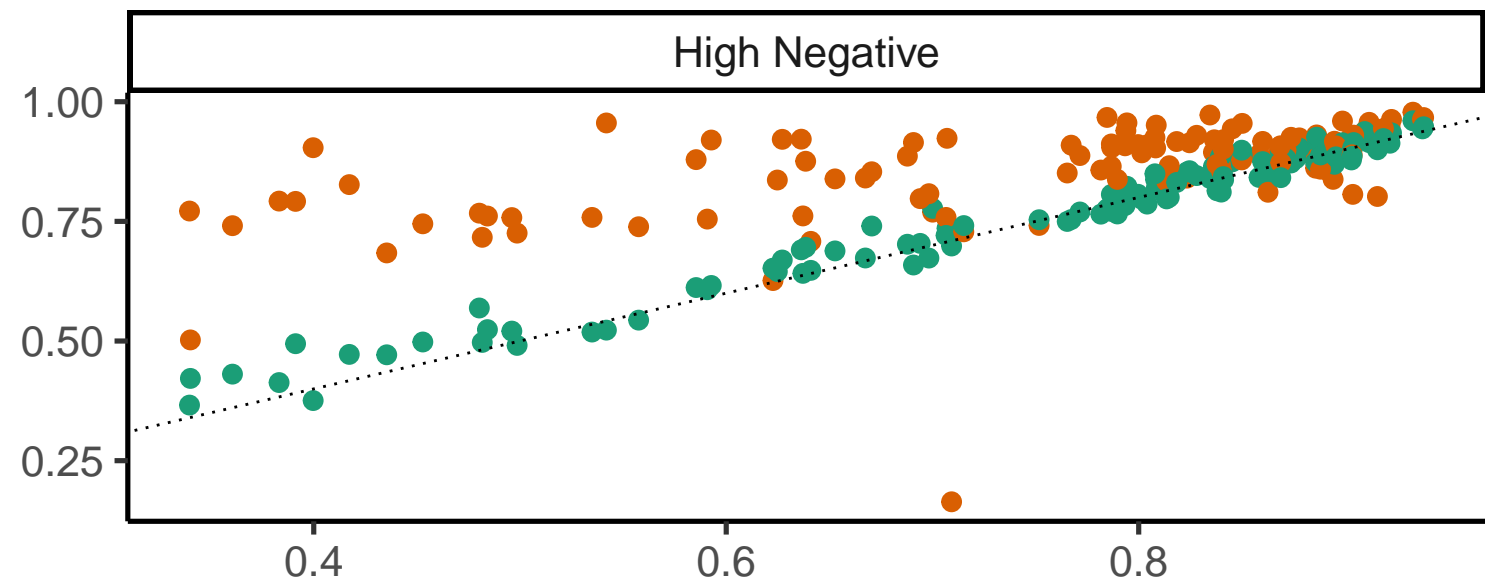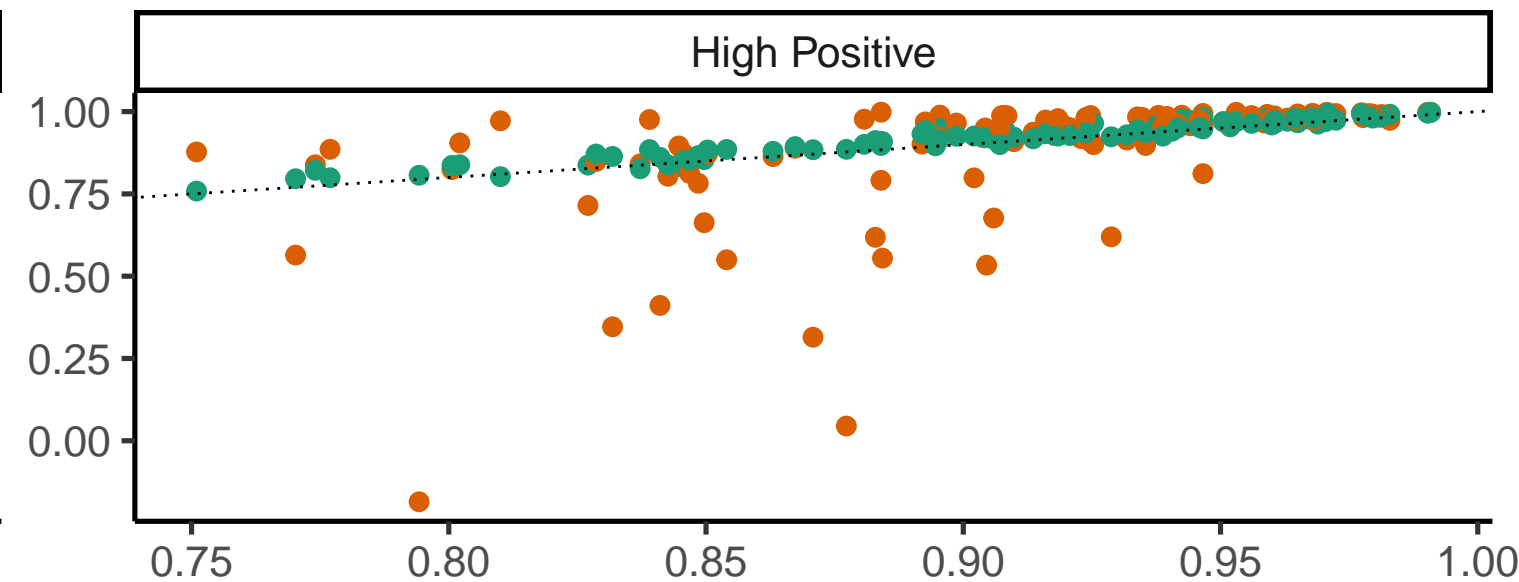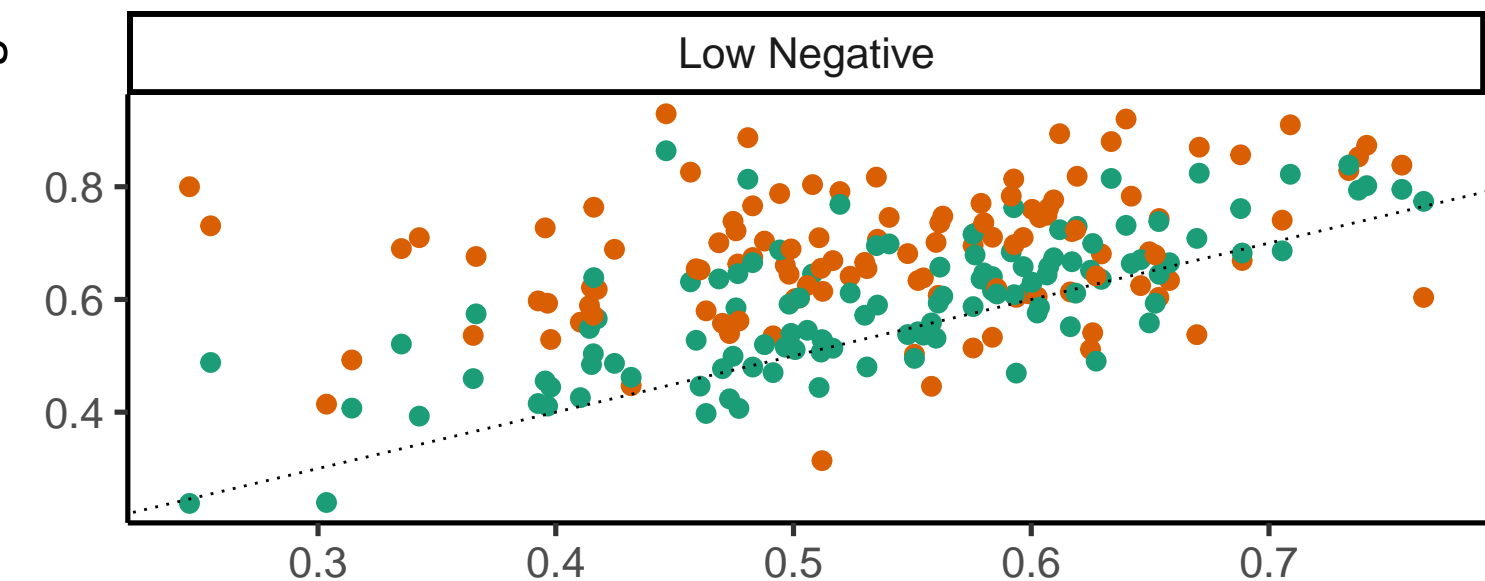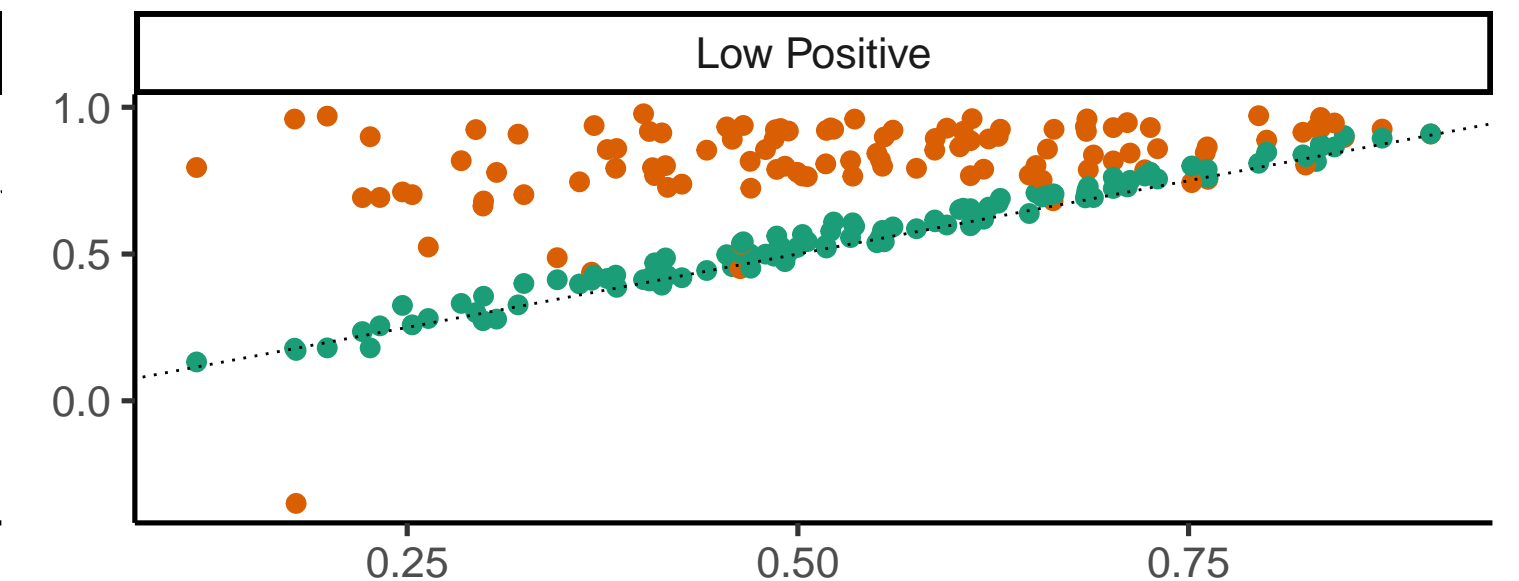

No Alignment

Method ● Penalized SRVF ● Unpenalized SRVF

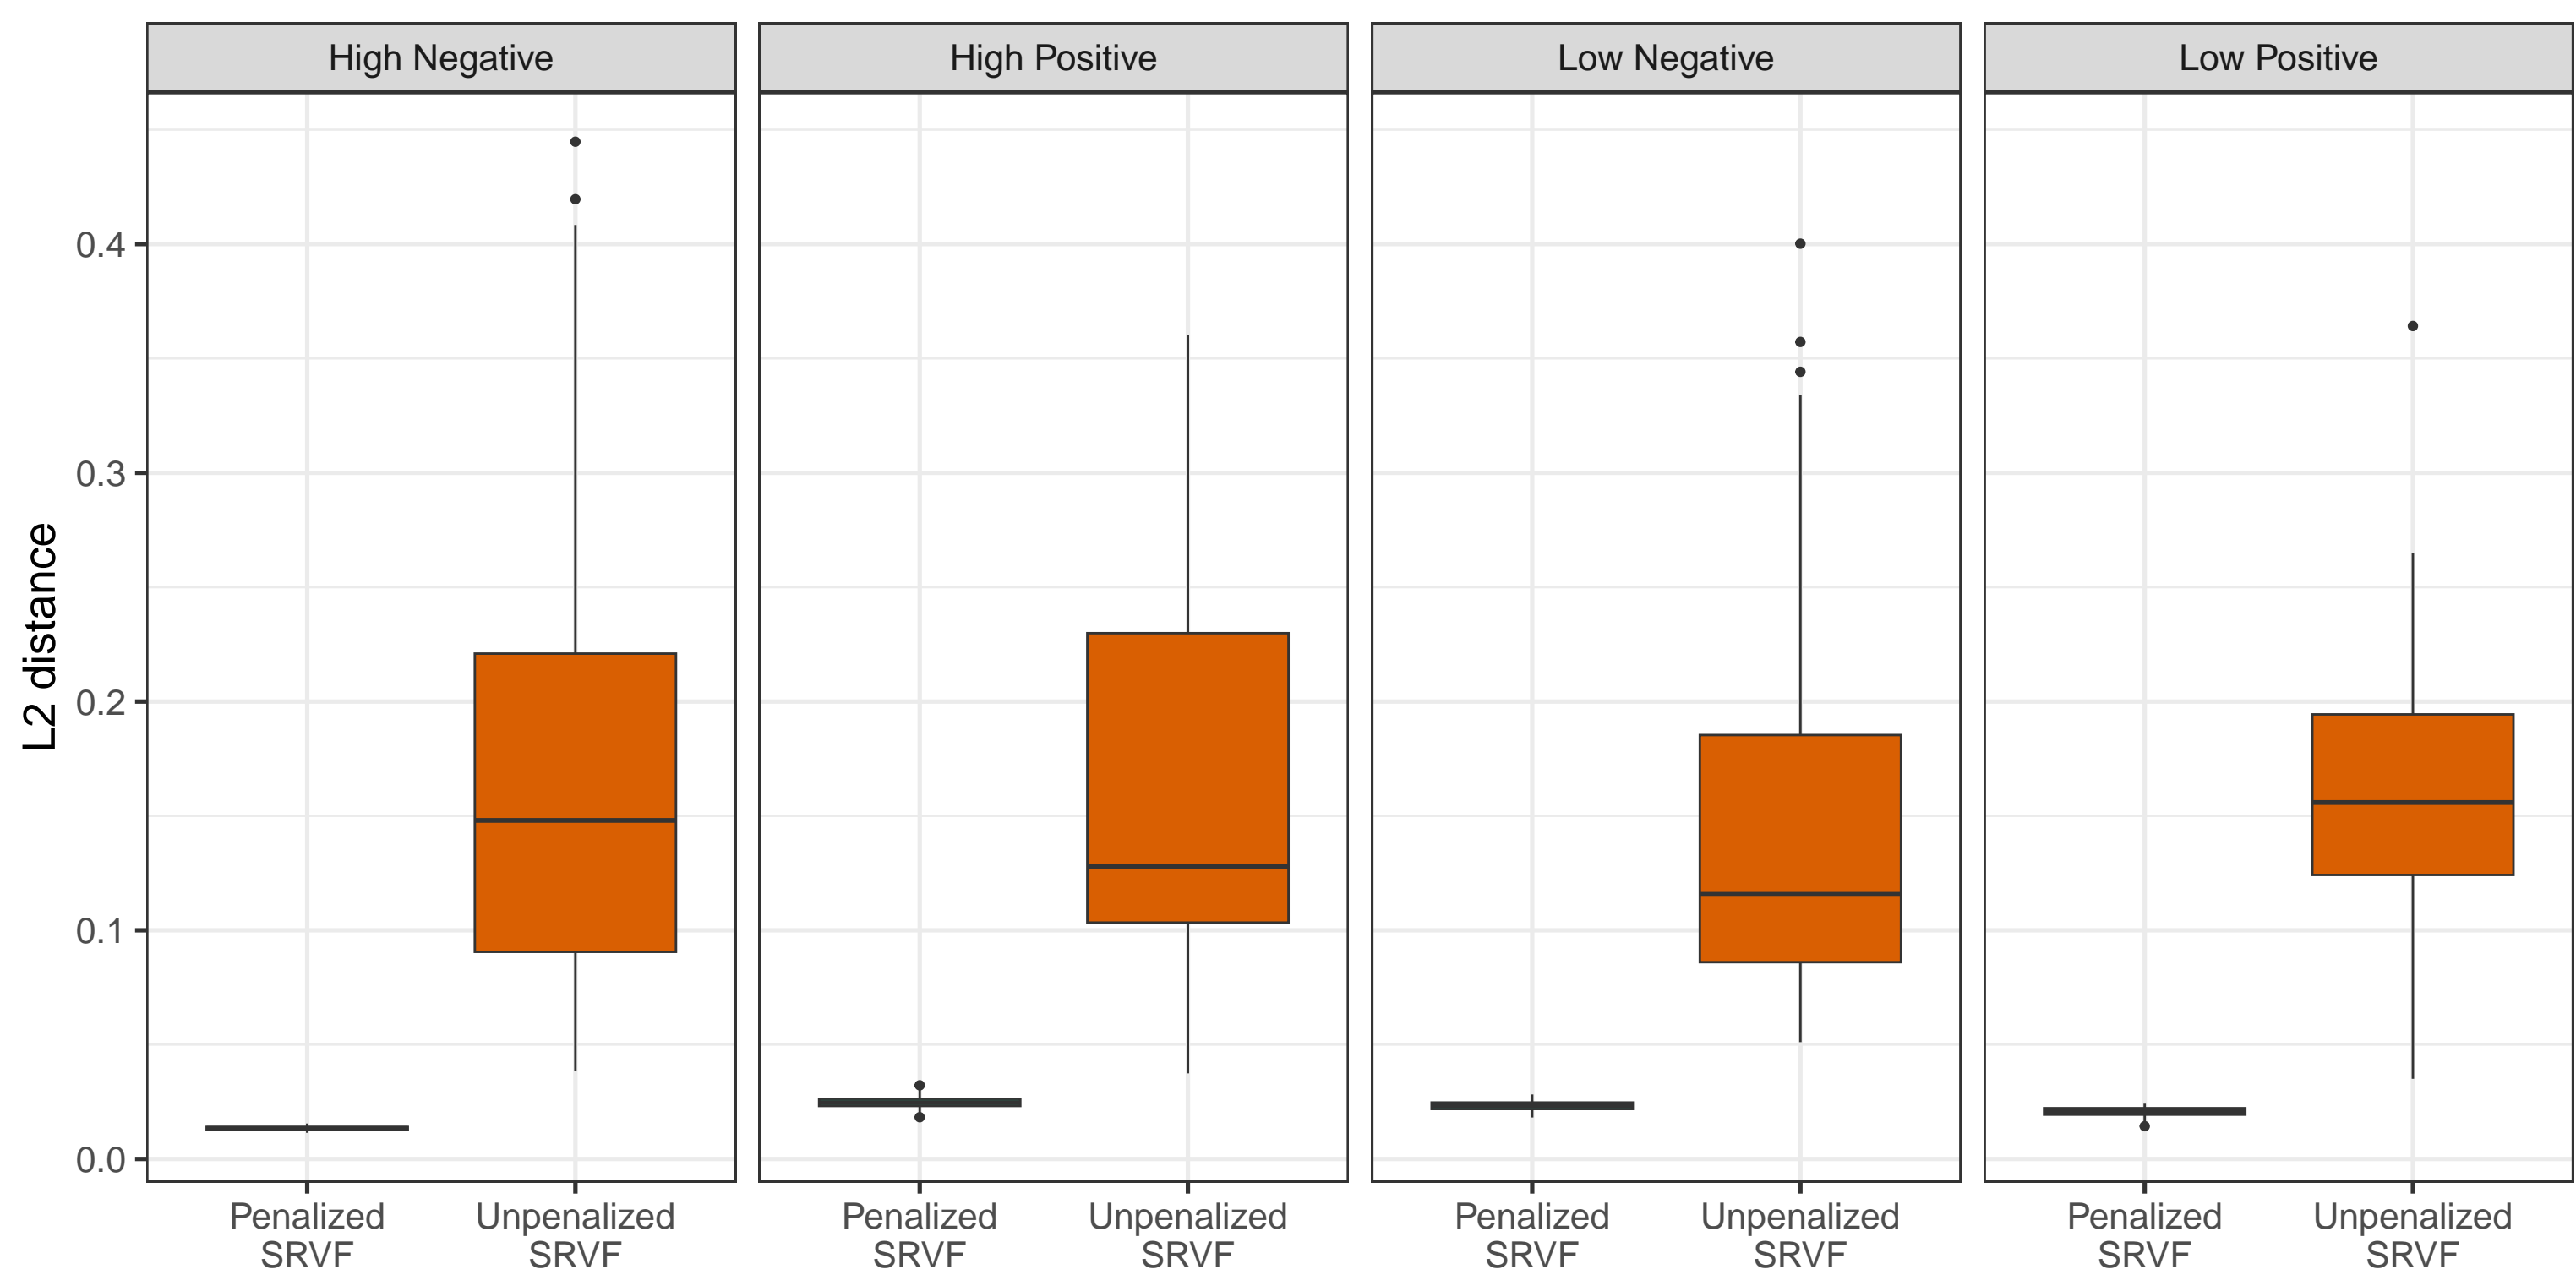

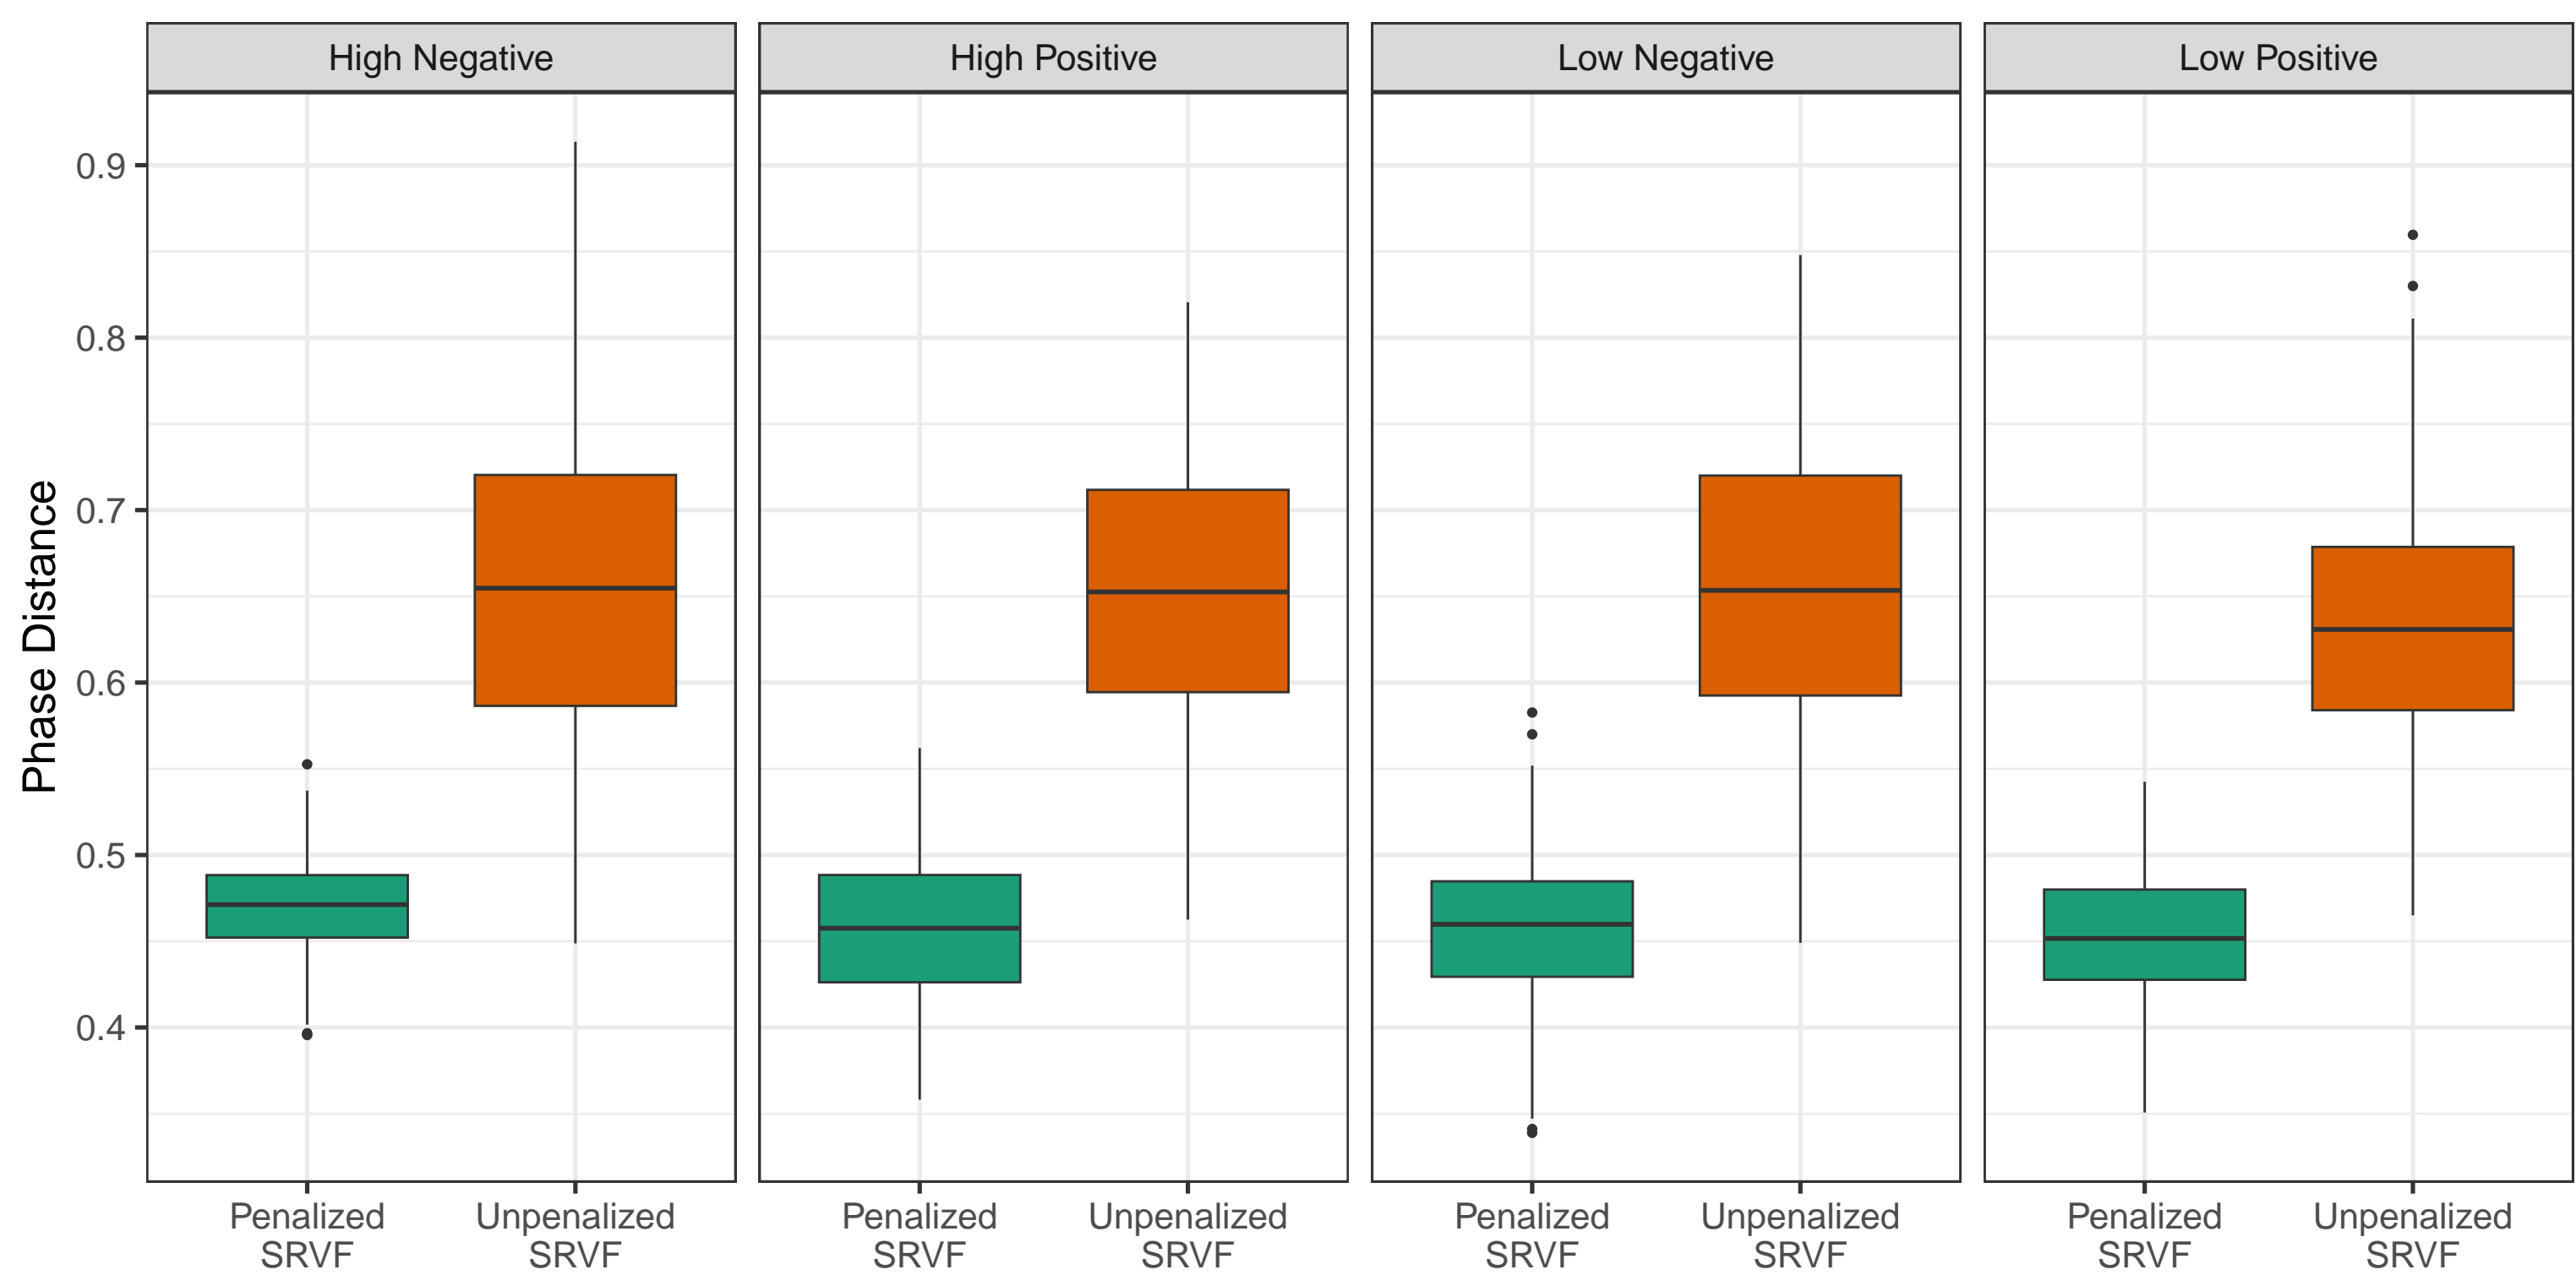

# Correlations on f

Alignment

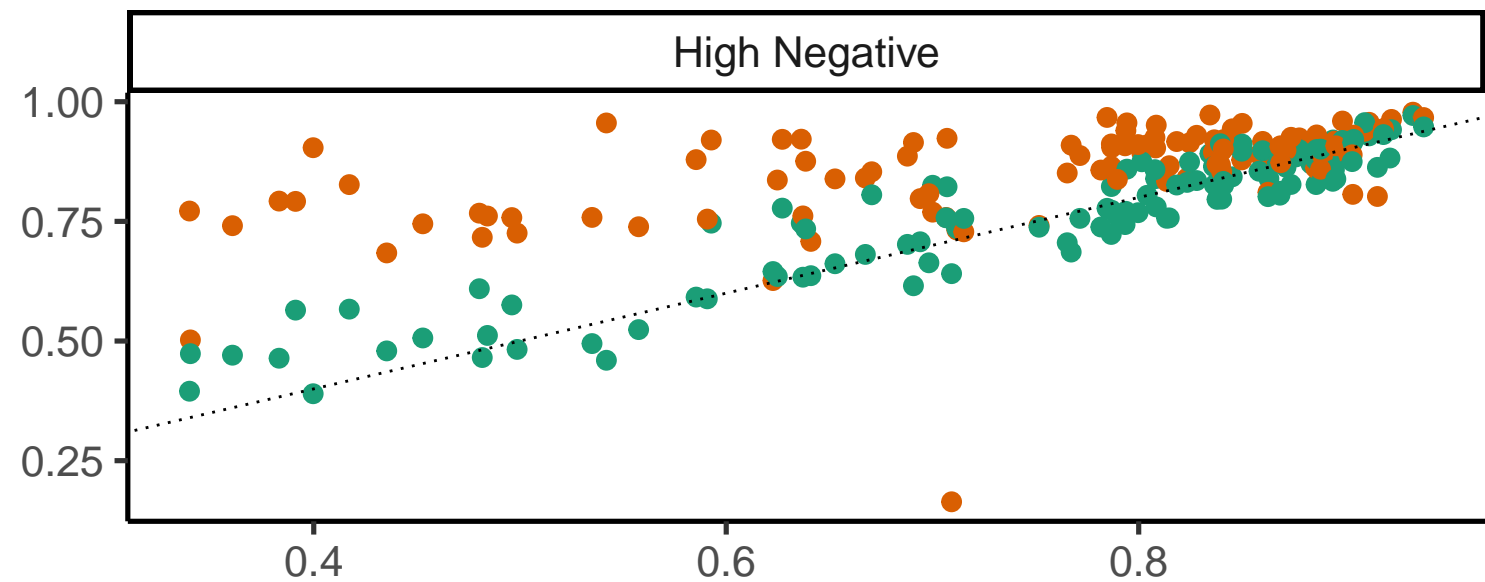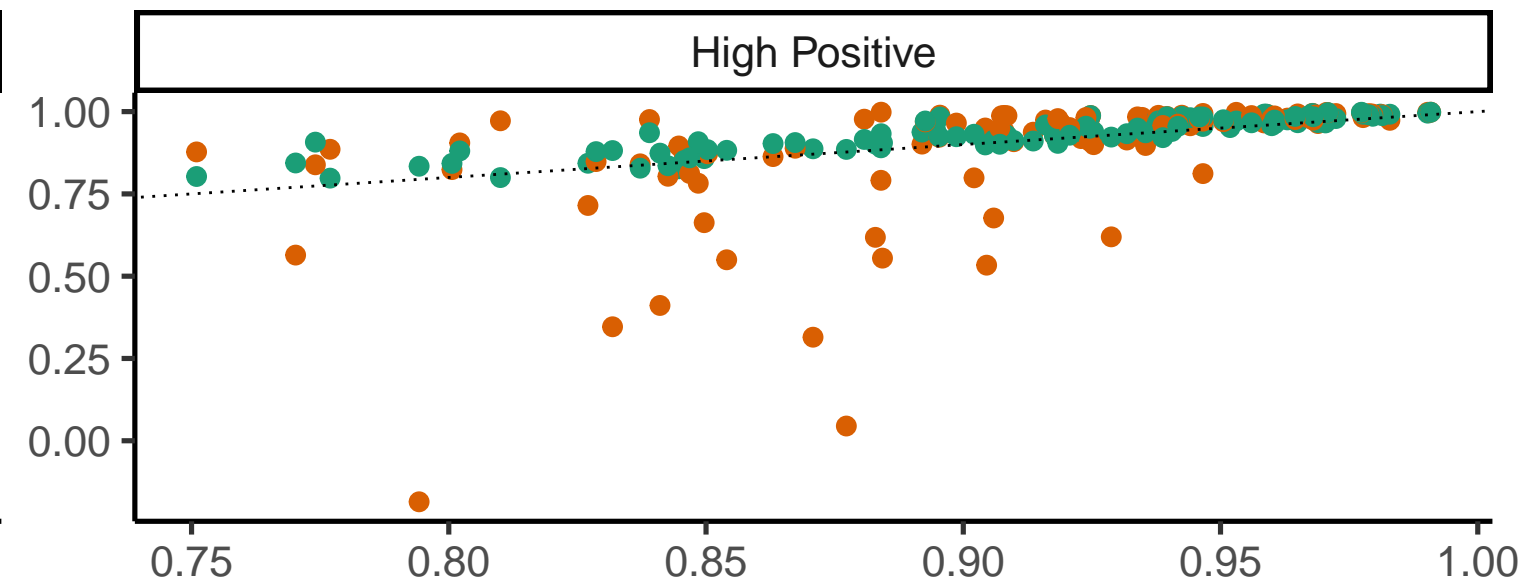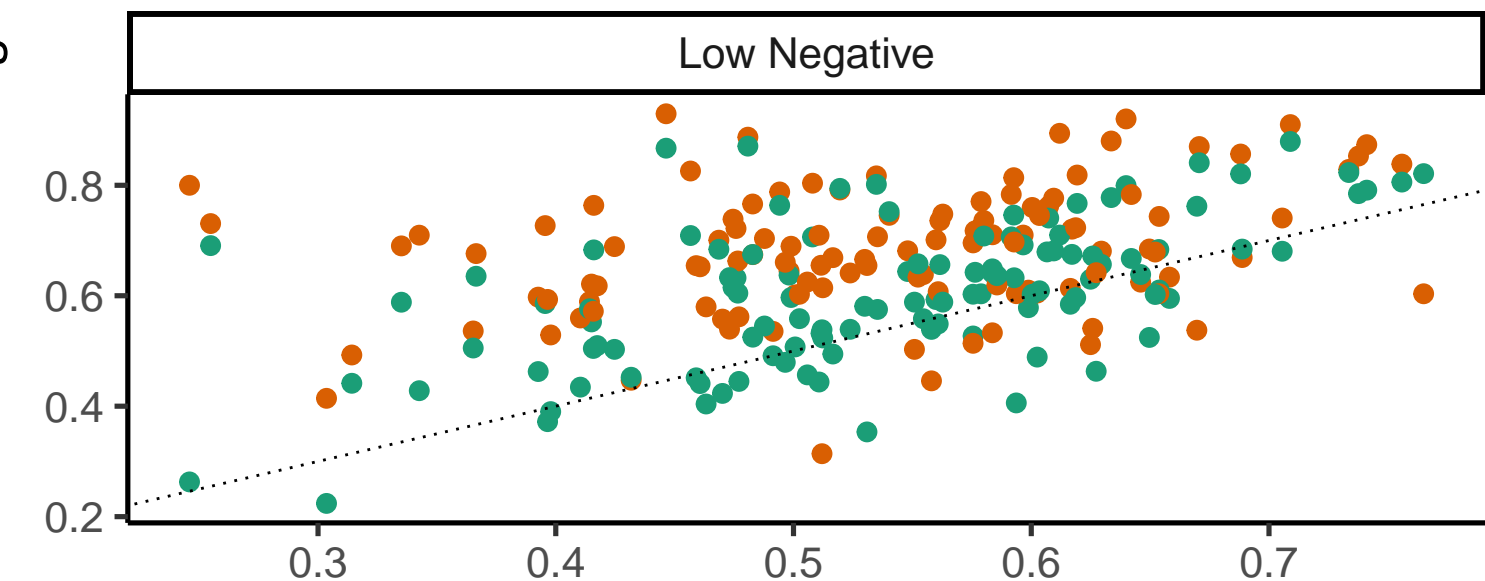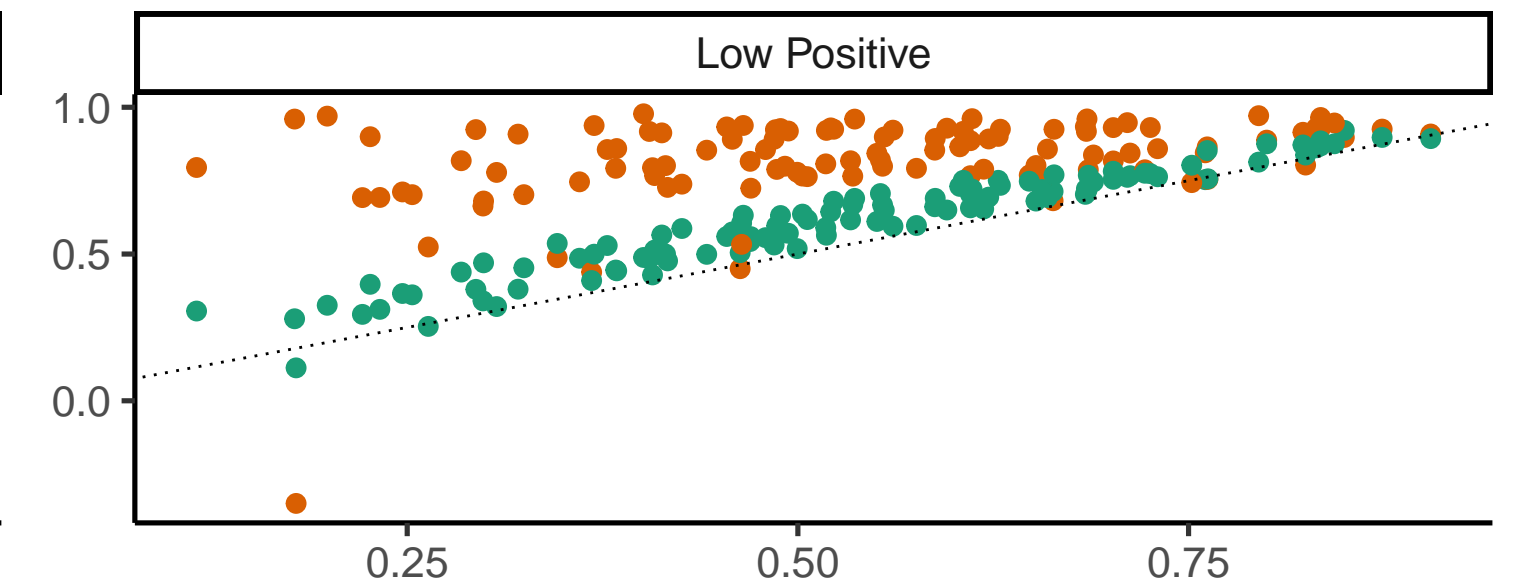

No Alignment

Method ● Penalized SRVF ● Unpenalized SRVF

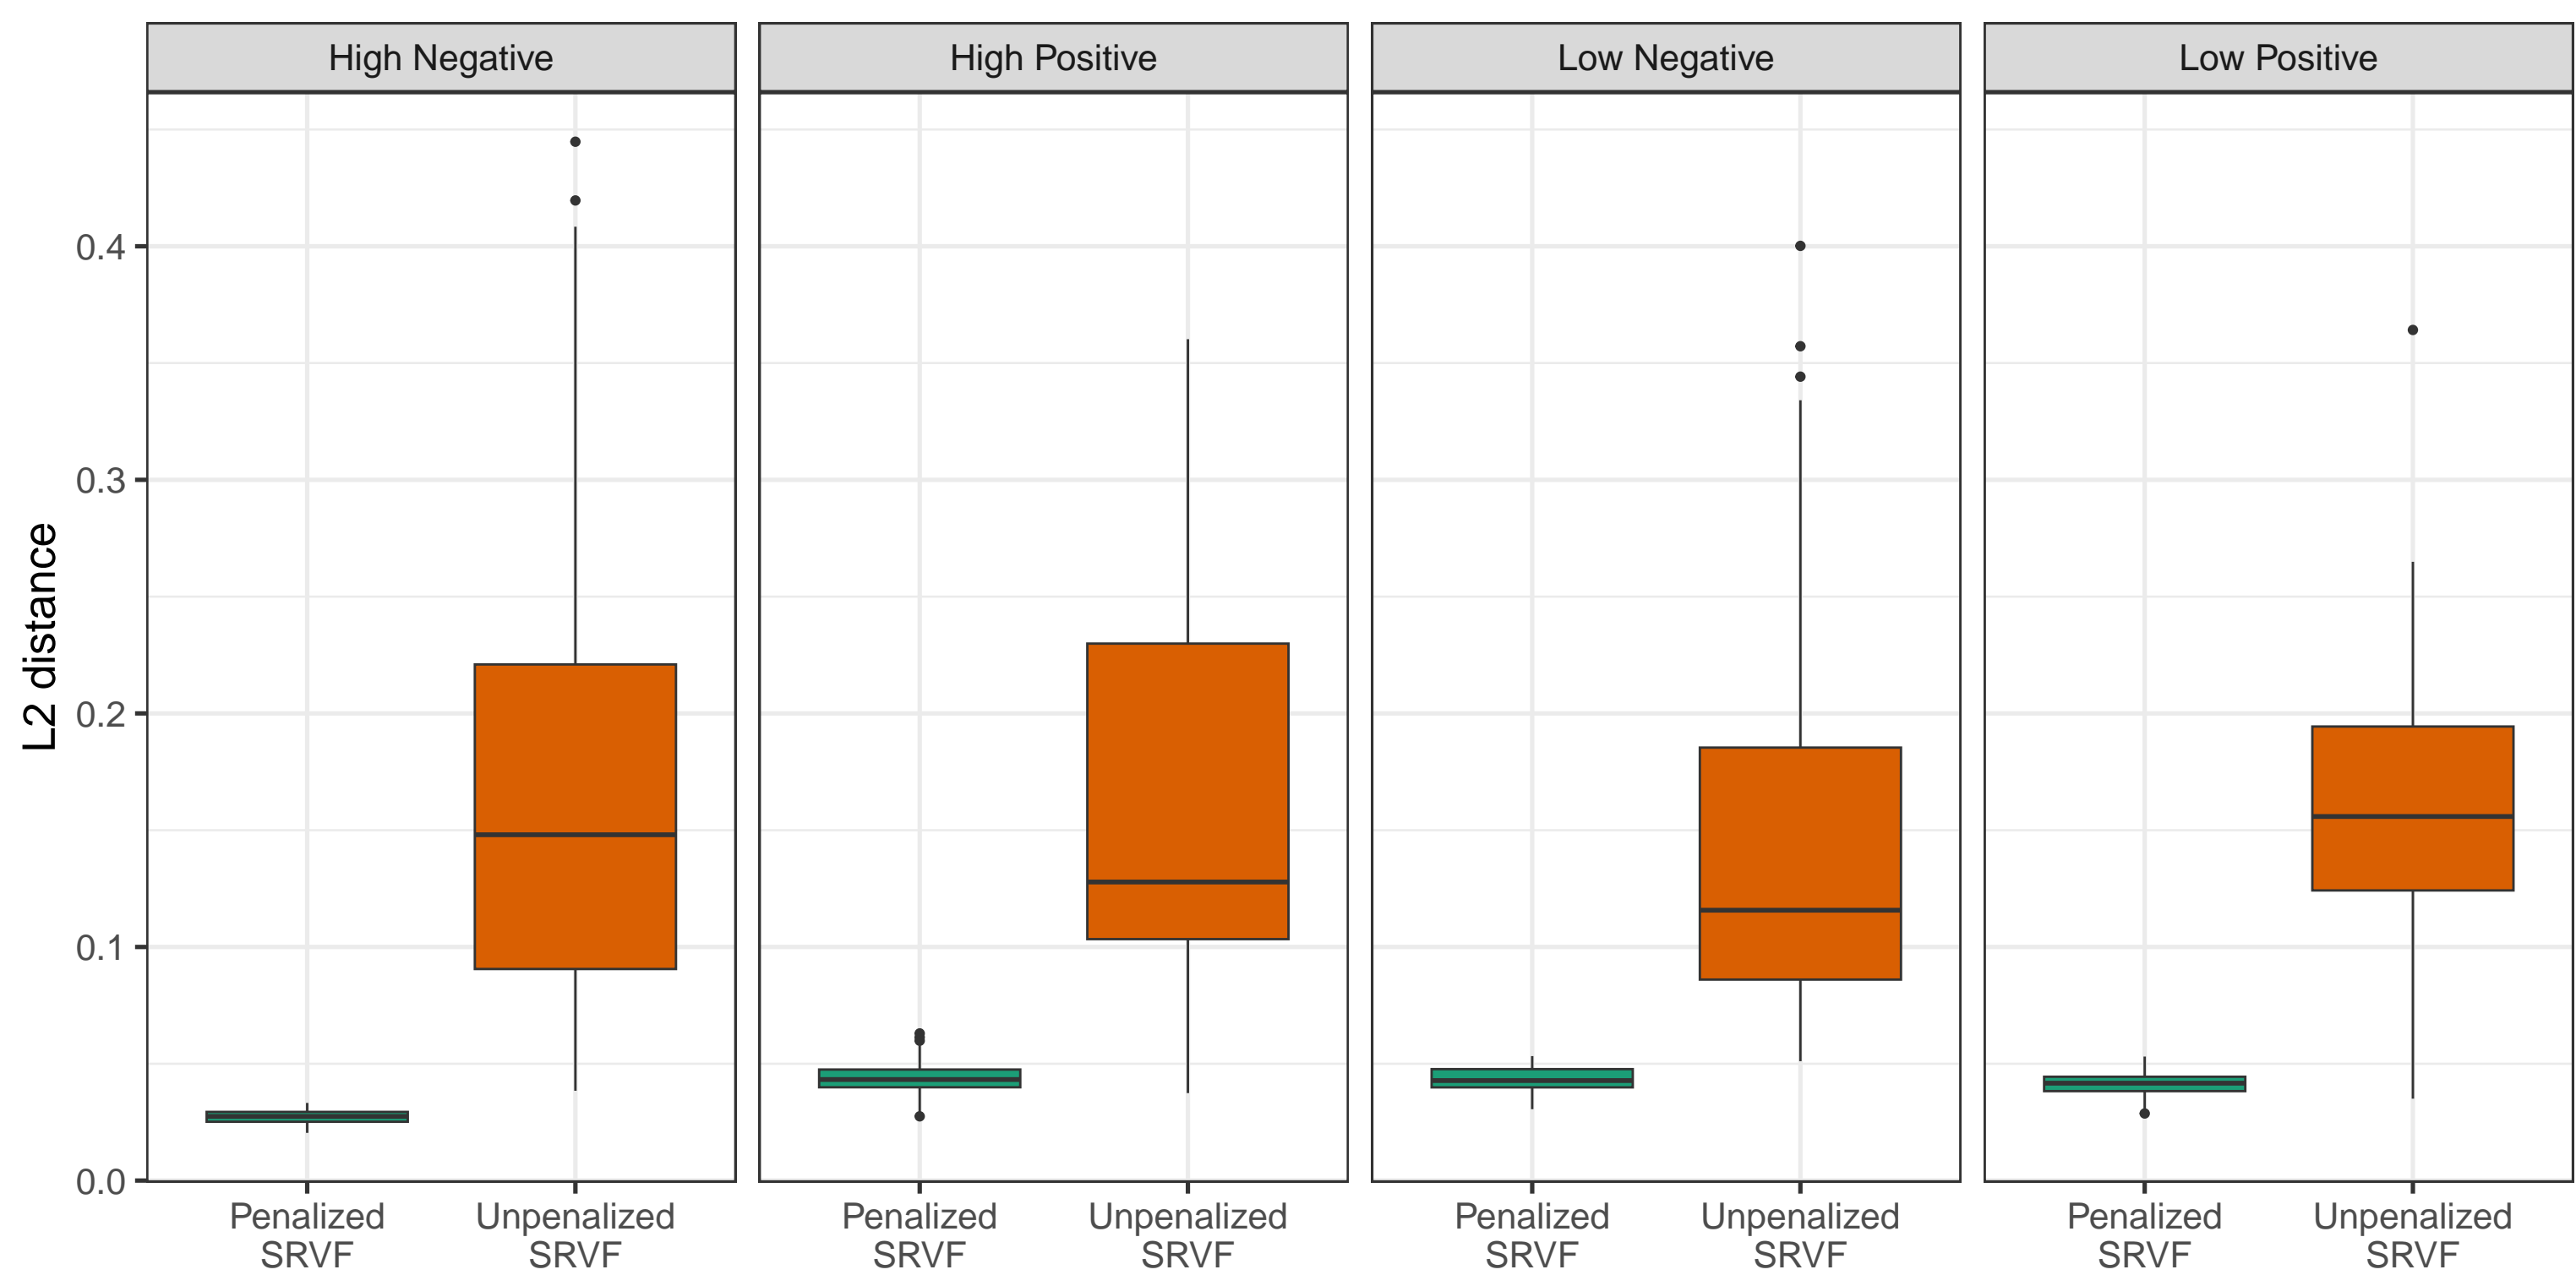

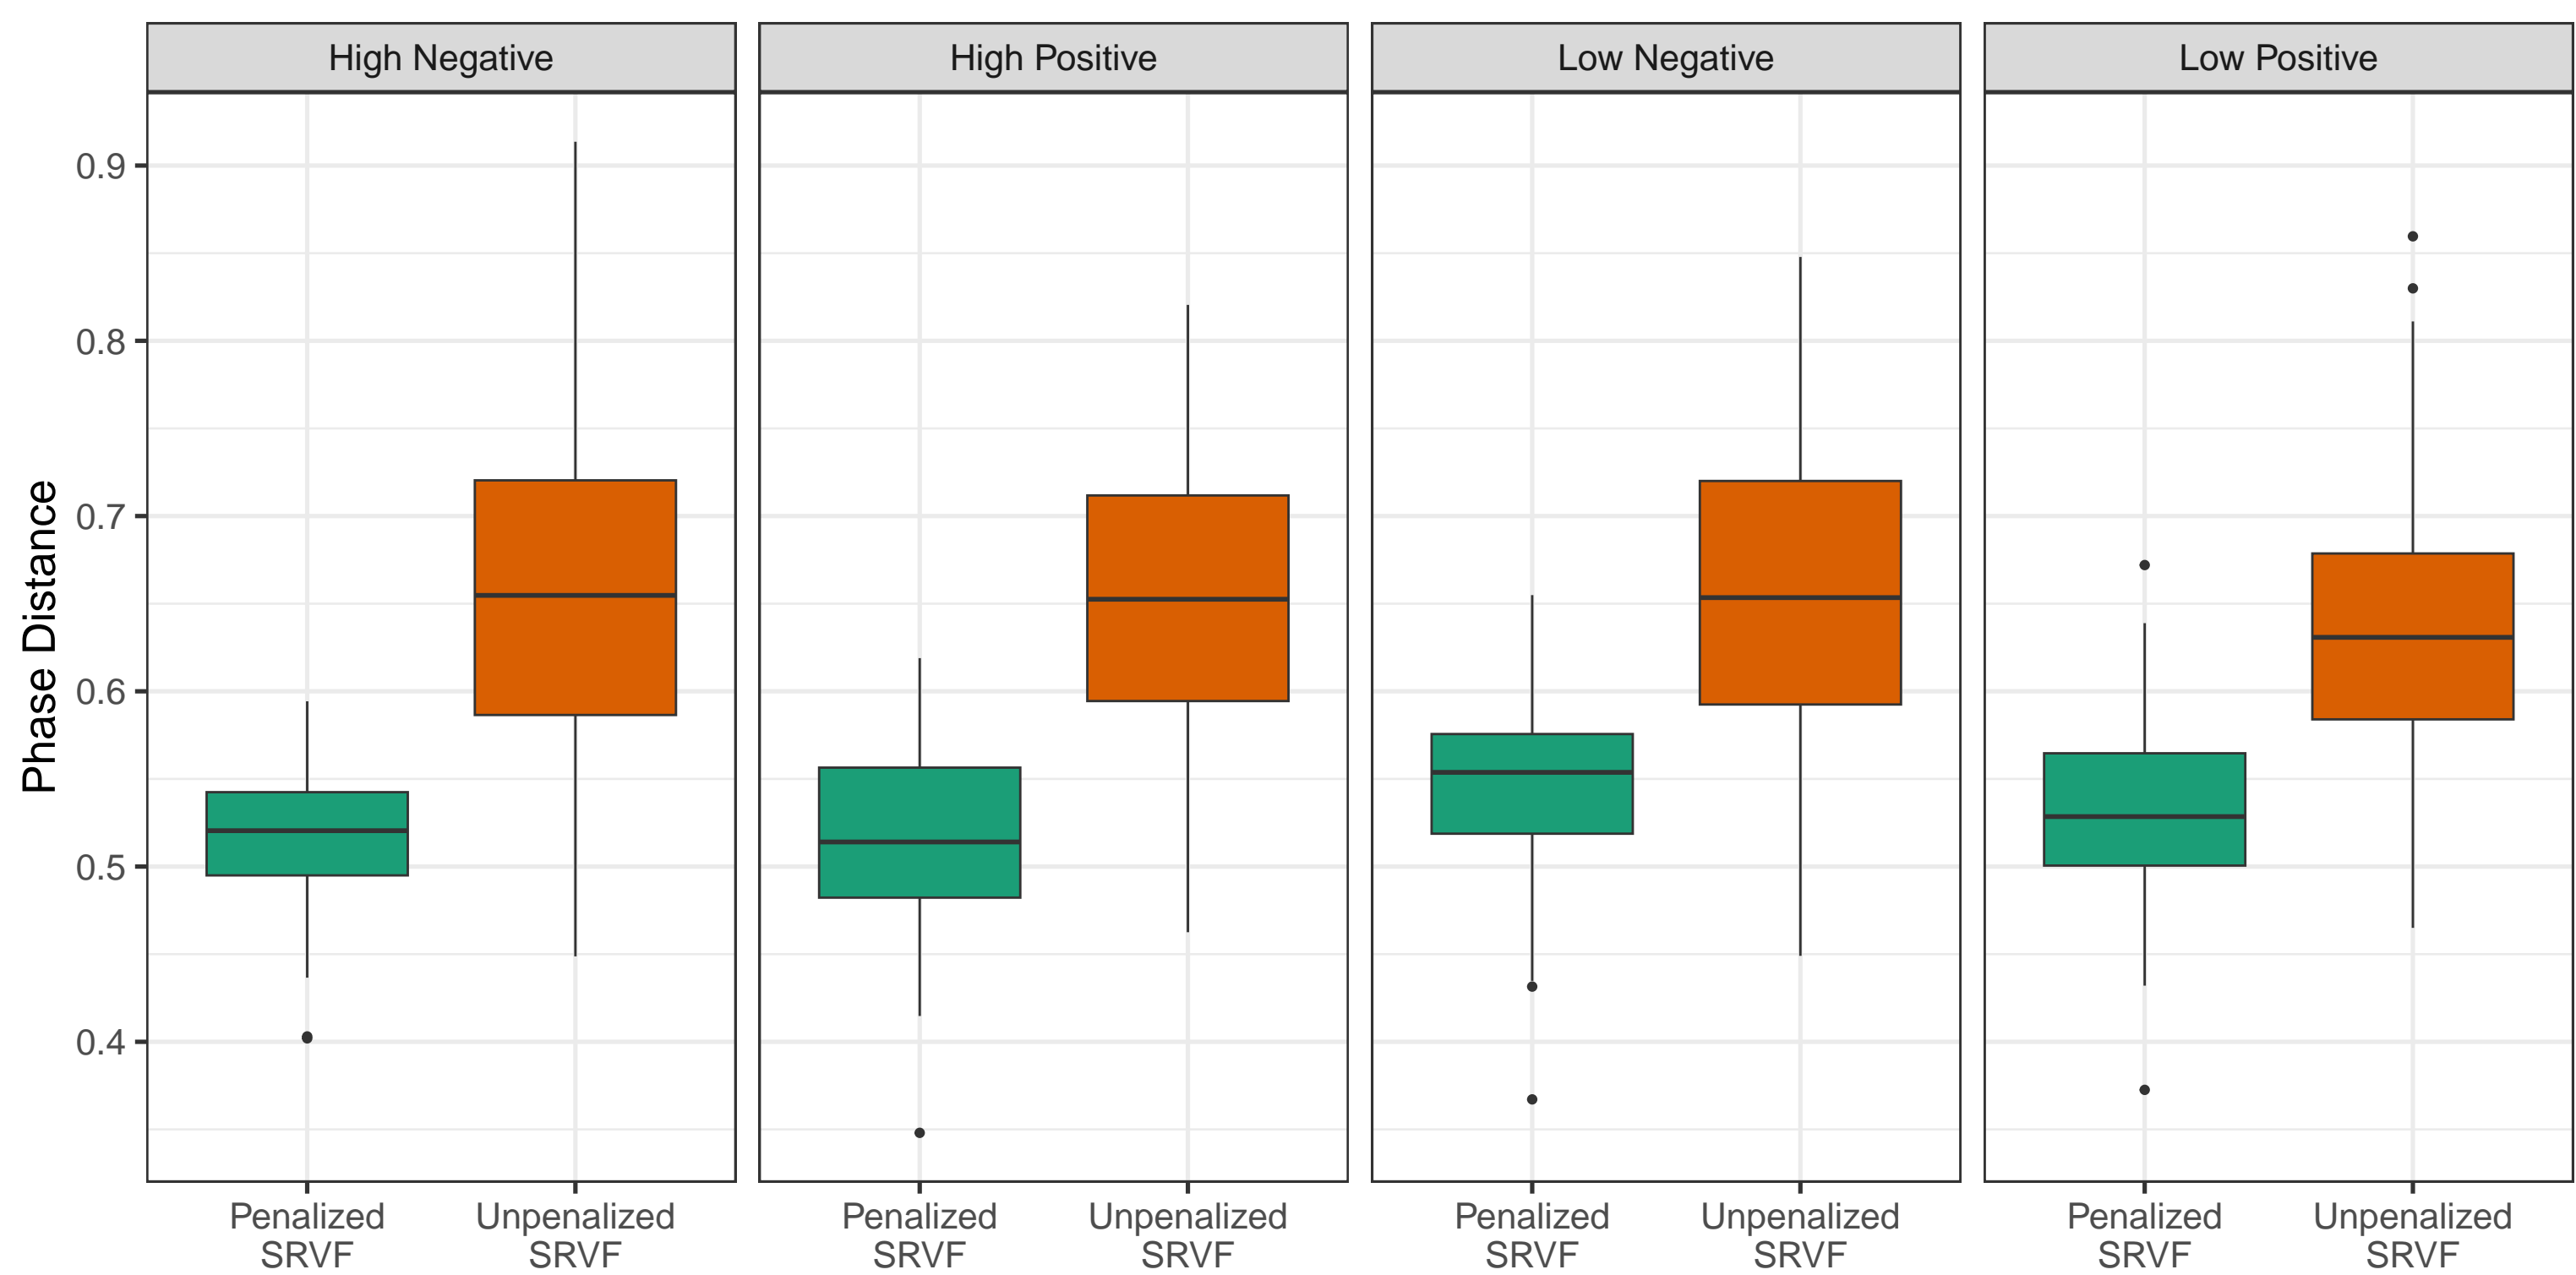

Supplement: Supplementary file 2 [file Delvin_new_plots_rmoutliers_22012024_appendix.pdf]
